# Supplementary material for: Triplet excitations in the frustrated spin ladder Li$_2$Cu$_2$O(SO$_4$)$_2$
Source: arXiv:1902.02798 ancillary file (2019-02-07)
Supplement: Supplementary file 1 [file Series.pdf]

(\* We report the perturbation matrix W, written in Mathematica, expressed in the  $|T\rangle_{\{\alpha\}}$  basis computed up to the fifth-order. \*)

(\* Here we use the nomenclature :\*)

(\*  $J^a \equiv J_a$  ;  $J_2 \equiv J_2$  ;  $J_x^b \equiv J_{dB}$  ;  $J_x^c \equiv J_{dC}$  ;  $J_{\perp}^a \equiv J_{pA}$  ;  $J_{\perp}^b \equiv J_{pB}$  \*)

(\* FIRST ORDER \*)

(\* The diagonal elements  $W_{11o1}$  and  $W_{22o1} = W_{11o1}$ , and the off-diagonal  $W_{12o1}$  and  $W_{21o1} = \text{Conjugate}[W_{12o1}]$  are, respectively: \*)

$$W_{11o1}[k_, Ja_, J2_, JdB_, JpA_, JpB_, JdC_] := \left( J_2 - \frac{J_a}{2} \right) \text{Cos}[k]$$

$$W_{12o1}[k_, Ja_, J2_, JdB_, JpA_, JpB_, JdC_] := \left( (\text{Cos}[k] - \text{Sin}[k] * i) * (2 * J_{dB} - J_{pA}) + 2 * J_{dC} - J_{pB} \right) / 4$$

(\* SECOND ORDER \*)

(\* The second-order expressions of the W's elements  $W_{11o2}$ ,  $W_{22o2} = W_{11o2}$ ,  $W_{12o2}$  and  $W_{21o2} = \text{Conjugate}[W_{12o2}]$  \*)

$$W_{11o2}[k_, Ja_, J2_, JdB_, JpA_, JpB_, JdC_] := \left( 12 * (J_{dC} - J_{pB}) * J_{dC} - (J_{pA}^2 + J_{pB}^2) + 12 * (J_{dB} - J_{pA}) * J_{dB} - 2 * J_a^2 + 24 * (J_2 - J_a) * J_2 - 2 * (2 * J_2 - J_a)^2 * \text{Cos}[2 * k] + 2 * ((2 * J_{dC} - J_{pB}) * J_{pA} - 4 * J_a^2 - 2 * (2 * J_{dC} - J_{pB}) * J_{dB}) * \text{Cos}[k] \right) / 32$$

$$W_{12o2}[k_, Ja_, J2_, JdB_, JpA_, JpB_, JdC_] := \left( 2 * (\text{Sin}[k] * i * J_{pA}^2 - J_{pB}^2) - (2 * J_2 - J_a) * (2 * J_{dB} - J_{pA}) - (\text{Cos}[2 * k] - \text{Sin}[2 * k] * i) * (2 * J_2 - J_a) * (2 * J_{dB} - J_{pA}) - 2 * ((2 * J_2 - J_a) * (2 * J_{dC} - J_{pB}) + J_{pA}^2) * \text{Cos}[k] \right) / 16$$

(\* THIRD ORDER \*)

(\* For the third-order expressions of the perturbation, diagonal elements are complex and one is the complex conjugate of the other, we thus have  $W_{11o3}, W_{22o3} = \text{Conjugate}[W_{11o3}]$ ,  $W_{12o3}$  and  $W_{21o3} = \text{Conjugate}[W_{12o3}]$  \*)

$$W_{11o3}[k_, Ja_, J2_, JdB_, JpA_, JpB_, JdC_] := \frac{1}{128} \left( 48 J_2^3 - 24 J_2^2 J_a + 6 J_a^3 + 24 J_{dB}^3 + 24 J_{dC}^3 - 12 J_{dB}^2 J_{pA} - 22 J_{dB} J_{pA}^2 + 3 J_{pA}^3 - 12 J_{dC}^2 J_{pB} - 22 J_{dC} J_{pB}^2 + 3 J_{pB}^3 - 4 J_2 (11 J_a^2 + 60 J_{dB} J_{dC} - 30 J_{dC} J_{pA} - 30 J_{dB} J_{pB} + 23 J_{pA} J_{pB}) + 2 J_a (2 J_{dB} (30 J_{dC} - 7 J_{pB}) + 7 J_{pA} (-2 J_{dC} + J_{pB})) - 2 (16 J_2^3 - 24 J_2^2 J_a - 2 J_a^3 + 2 J_{dC} (4 J_{dB} (J_{dB} + J_{dC}) - 2 J_{dC} J_{pA} + J_{pA}^2) + (-4 J_{dB}^2 - 4 (J_{dB} + J_{dC}) J_{pA} + J_{pA}^2) J_{pB} + (2 J_{dB} + J_{pA}) J_{pB}^2 - J_a (4 J_{dB}^2 + 4 J_{dB} J_{dC} + 4 J_{dC}^2 - 4 J_{dB} J_{pA} + 10 J_{dC} J_{pA} + 5 J_{pA}^2 + 10 J_{dB} J_{pB} - 4 J_{dC} J_{pB} - 7 J_{pA} J_{pB} + 5 J_{pB}^2) + 2 J_2 (14 J_a^2 + 4 J_{dB}^2 + 4 J_{dC}^2 + 2 J_{dC} J_{pA} + 5 J_{pA}^2 - 4 J_{dC} J_{pB} + 3 J_{pA} J_{pB} + 5 J_{pB}^2 + 2 J_{dB} (-2 (J_{dC} + J_{pA}) + J_{pB})) \right) \text{Cos}[k] - 2 (2 J_2 - J_a) (8 J_2^2 - 2 J_a^2 - 3 (2 J_{dB} - J_{pA}) (2 J_{dC} - J_{pB})) \text{Cos}[2 k] + 2 (2 J_2 - J_a)^3 \text{Cos}[3 k] + 4 i (2 J_{dC} J_{pA}^2 + J_{pB} (-2 J_{dB} J_{pB} + J_{pA} (-J_{pA} + J_{pB}))) \text{Sin}[k]$$

$$\begin{aligned}
W12o3[k_, Ja_, J2_, JdB_, JpA_, JpB_, JdC_] := & \\
& \frac{1}{128} \left( 3 e^{-3 i k} (-2 J2 + Ja)^2 (2 JdB - JpA) + 8 J2^2 (-2 JdB - 2 JdC + JpA + JpB) + \right. \\
& 2 Ja^2 (-2 JdB - 10 JdC + 3 JpA + 5 JpB) + \\
& 2 Ja (4 JdB^2 - 4 JdB (JdC + JpA) + JpA (10 JdC + 3 JpA - 3 JpB) + 10 JdB JpB) - \\
& 2 (-8 JdB JdC JpA + 6 JdC JpA^2 + JdB^2 (8 JdC - 4 JpB) - JpA^2 JpB + 8 JdC JpB^2) - 4 J2 \\
& (4 JdB^2 - 2 JdB (2 JdC + JpB) + 2 Ja (-2 JdC + JpA + JpB) + JpA (2 JdC + JpA + 7 JpB)) - \\
& (Ja^2 (14 JdB + 8 JdC - 7 JpA - 4 JpB) + \\
& 4 J2^2 (-2 JdB + 8 JdC + JpA - 4 JpB) - JpA (2 JdC + JpB)^2 - \\
& 2 Ja (-4 JdB JdC + 8 JdC^2 + 10 JdC JpA + 10 JdB JpB - 3 JpA JpB + 2 JpB^2) + \\
& 4 J2 (Ja (2 JdB - JpA) - 2 JdC (2 JdB - 4 JdC + JpA) + (2 JdB + 7 JpA) JpB + 2 JpB^2) + \\
& \left. 2 JdB (8 JpA^2 + 4 JdC (JdC - JpB) + 5 JpB^2) \right) \text{Cos}[k] + \\
& (Ja (8 JdB^2 + 8 JdB JpA - 2 JpA^2) + 8 J2^2 (-2 JdB + 6 JdC + JpA - 3 JpB) + \\
& (-2 JdB + JpA)^2 (2 JdC - JpB) - 2 Ja^2 (2 JdB - 6 JdC + JpA + 3 JpB) - \\
& 4 J2 (4 JdB^2 + 12 Ja JdC - 2 Ja JpA + JpA^2 - 6 Ja JpB)) \text{Cos}[2 k] + \\
& i (20 J2^2 (2 JdB - JpA) + Ja^2 (26 JdB - 13 JpA - 8 JpB) + \\
& 2 Ja (4 JdB JdC - 10 JdC JpA - 10 JdB JpB + 8 JdC JpB + 3 JpA JpB - 4 JpB^2) + \\
& JpA (-12 JdC^2 + 4 JdC JpB - 3 JpB^2) + 2 JdB (8 JpA^2 + 12 JdC (JdC - JpB) + 7 JpB^2) + \\
& 4 J2 (-2 JdC JpA + 7 JpA JpB + 2 JdB (-2 JdC + JpB) + Ja (-10 JdB + 5 JpA + 4 JpB))) \\
& \text{Sin}[k] - i (8 J2^2 (-2 JdB + JpA) - 2 Ja^2 (2 JdB + JpA) + Ja (8 JdB^2 + 8 JdB JpA - 2 JpA^2) - \\
& 4 J2 (4 JdB^2 + JpA (-2 Ja + JpA)) + (-2 JdB + JpA)^2 (2 JdC - JpB)) \text{Sin}[2 k]
\end{aligned}$$

(\* FOURTH ORDER \*)

(\* The results of the fourth-order expressions W11o4,

W22o4=Conjugate[W11o4],W12o4 and W21o4=Conjugate[W12o4] are \*)

$$W11o4[k_, Ja_, J2_, JdB_, JpA_, JpB_, JdC_] :=$$

$$\begin{aligned}
& \frac{1}{6144} \left( 3 (-416 J2^4 + 1344 J2^3 Ja + 46 Ja^4 + 48 JdB^4 - 512 JdB^2 JdC^2 + 48 JdC^4 + \right. \\
& 288 JdB^3 JpA + 384 JdB JdC^2 JpA - 568 JdB^2 JpA^2 - 224 JdC^2 JpA^2 + \\
& 72 JdB JpA^3 + 67 JpA^4 + 16 JdC (24 JdB^2 + 18 JdC^2 + 2 JdB JpA + 7 JpA^2) JpB - \\
& 8 (28 JdB^2 + 71 JdC^2 - 14 JdB JpA + 11 JpA^2) JpB^2 + 72 JdC JpB^3 + 67 JpB^4 + \\
& 4 Ja^2 (28 JdB^2 + 28 JdC^2 - 56 JdC JpA - 13 JpA^2 + 4 JdB (34 JdC - 11 JpA - 14 JpB) - \\
& 44 JdC JpB + 18 JpA JpB - 13 JpB^2) - 16 J2^2 (97 Ja^2 - 76 JdB^2 - 76 JdC^2 - 44 JdC \\
& JpA - 7 JpA^2 + JdB (72 JdC + 92 JpA - 44 JpB) + 92 JdC JpB + 38 JpA JpB - 7 JpB^2) + \\
& 8 Ja (4 JdB^2 (22 JdC + JpB) + 4 JdB (22 JdC^2 + 9 JdC (JpA + JpB) - 7 JpB (JpA + JpB)) + \\
& JpA (4 JdC^2 - 28 JdC (JpA + JpB) + 15 JpB (JpA + JpB))) + \\
& 16 J2 (23 Ja^3 - 72 JdB JdC (JdB + JdC) + 4 JdC (-2 JdB + 11 JdC) JpA + \\
& 34 JdC JpA^2 - 2 (-22 JdB^2 + 4 JdB JdC + 13 (JdB + JdC) JpA + 8 JpA^2) JpB + \\
& 2 (17 JdB - 8 JpA) JpB^2 - Ja (92 JdB^2 + 92 JdC^2 + 11 JpA^2 + 4 JpA JpB + \\
& 11 JpB^2 - 18 JdC (JpA + 6 JpB) + 2 JdB (4 JdC - 9 (6 JpA + JpB)))) - \\
& 4 (480 J2^4 - 480 J2^3 Ja - 30 Ja^4 + 2 Ja^2 (52 JdB^2 - 82 JdB JdC + 52 JdC^2 - \\
& 52 JdB JpA + 125 JdC JpA + 33 JpA^2) + 6 JdC (-8 JdB (JdB^2 - 3 JdB JdC + JdC^2) + \\
& 4 (11 JdB^2 + JdC^2) JpA + 2 (JdB - 3 JdC) JpA^2 + 5 JpA^3) - \\
& \left. 4 Ja (24 (JdB^3 + JdC^3) + 4 (-3 JdB^2 + 26 JdB JdC + 14 JdC^2) JpA + \right.
\end{aligned}$$

$$\begin{aligned}
& 2 (15 \text{JdB} - 13 \text{JdC}) \text{JpA}^2 + 9 \text{JpA}^3) + (\text{Ja}^2 (250 \text{JdB} - 104 \text{JdC} - 105 \text{JpA}) + \\
& 8 \text{Ja} (-28 \text{JdB}^2 - 52 \text{JdB JdC} + 6 \text{JdC}^2 + 11 \text{JdB JpA} + 11 \text{JdC JpA} + 8 \text{JpA}^2) + \\
& 3 (8 \text{JdB} (\text{JdB}^2 + 11 \text{JdC}^2) - 28 (3 \text{JdB}^2 - 2 \text{JdB JdC} + 3 \text{JdC}^2) \text{JpA} + \\
& \quad 6 (\text{JdB} - 6 \text{JdC}) \text{JpA}^2 + \text{JpA}^3)) \text{JpB} + (66 \text{Ja}^2 + 8 \text{Ja} (13 \text{JdB} - 15 \text{JdC} + 8 \text{JpA}) + \\
& 3 (-12 \text{JdB}^2 + 4 \text{JdB} (\text{JdC} - 9 \text{JpA}) + \text{JpA} (6 \text{JdC} + 13 \text{JpA})) \text{JpB}^2 + \\
& 3 (-12 \text{Ja} + 10 \text{JdB} + \text{JpA}) \text{JpB}^3 + 4 \text{J}^2 (144 \text{Ja}^2 + 72 \text{JdB}^2 + 72 \text{JdC}^2 + 186 \text{JdC JpA} + \\
& \quad 82 \text{JpA}^2 - 6 \text{JdB} (62 \text{JdC} + 12 \text{JpA} - 31 \text{JpB}) - 72 \text{JdC JpB} + 35 \text{JpA JpB} + 82 \text{JpB}^2) + \\
& 4 \text{J}^2 (-6 (9 \text{Ja}^3 - 66 \text{Ja JdB JdC} - 4 (\text{JdB} - 2 \text{JdC}) (2 \text{JdB} - \text{JdC}) (\text{JdB} + \text{JdC})) - \\
& \quad 6 (4 \text{JdB}^2 + 57 \text{Ja JdC} - 6 \text{JdB JdC}) \text{JpA} - 4 (16 \text{Ja} - 15 \text{JdB} + 2 \text{JdC}) \text{JpA}^2 + 18 \text{JpA}^3 + \\
& \quad (12 (3 \text{JdB} - 2 \text{JdC}) \text{JdC} + 142 (\text{JdB} + \text{JdC}) \text{JpA} - 43 \text{JpA}^2 + \text{Ja} (-342 \text{JdB} + 115 \\
& \quad \text{JpA})) \text{JpB} - (64 \text{Ja} + 8 \text{JdB} - 60 \text{JdC} + 43 \text{JpA}) \text{JpB}^2 + 18 \text{JpB}^3) \text{Cos}[k] - \\
& 2 (96 \text{J}^2 + 1152 \text{J}^3 \text{Ja} + 90 \text{Ja}^4 + 15 (-2 \text{JdB} + \text{JpA})^2 (-2 \text{JdC} + \text{JpB})^2 - \\
& \quad 8 \text{J}^2 (96 \text{Ja}^2 - 36 \text{JdB}^2 - 36 \text{JdC}^2 - 48 \text{JdC JpA} - 29 \text{JpA}^2 + \\
& \quad 12 \text{JdB} (8 \text{JdC} + 3 \text{JpA} - 4 \text{JpB}) + 36 \text{JdC JpB} - 48 \text{JpA JpB} - 29 \text{JpB}^2) + \\
& 16 \text{Ja} (\text{JdC} (12 \text{JdB} (\text{JdB} + \text{JdC}) - 2 (\text{JdB} + \text{JdC}) \text{JpA} - 7 \text{JpA}^2) - \\
& \quad 2 (\text{JdB}^2 + (\text{JdC} - 2 \text{JpA}) \text{JpA} + \text{JdB} (\text{JdC} + \text{JpA})) \text{JpB} + (-7 \text{JdB} + 4 \text{JpA}) \text{JpB}^2) + \\
& \text{Ja}^2 (8 \text{JdB}^2 + 8 \text{JdC}^2 + 42 \text{JpA}^2 + 8 \text{JdB} (88 \text{JdC} - \text{JpA} - 12 \text{JpB}) + \\
& \quad 64 \text{JpA JpB} + 42 \text{JpB}^2 - 8 \text{JdC} (12 \text{JpA} + \text{JpB})) + \\
& 8 \text{J}^2 (-30 \text{Ja}^3 + 8 \text{JdC} (-6 \text{JdB} (\text{JdB} + \text{JdC}) + 3 \text{JdC JpA} + 4 \text{JpA}^2) + \\
& \quad 2 (12 \text{JdB}^2 - 2 (\text{JdB} + \text{JdC}) \text{JpA} - 7 \text{JpA}^2) \text{JpB} + 2 (16 \text{JdB} - 7 \text{JpA}) \text{JpB}^2 - \\
& \quad \text{Ja} (36 \text{JdB}^2 + 36 \text{JdC}^2 - 36 \text{JdB JpA} + 64 \text{JdC JpA} + 29 \text{JpA}^2 + \\
& \quad 64 \text{JdB JpB} - 36 \text{JdC JpB} + 8 \text{JpA JpB} + 29 \text{JpB}^2)) \text{Cos}[2k] + \\
& 4 (-2 \text{J}^2 + \text{Ja})^2 (48 \text{J}^2 - 32 \text{Ja}^2 - 45 (2 \text{JdB} - \text{JpA}) (2 \text{JdC} - \text{JpB})) \\
& \text{Cos}[3k] - 30 \\
& (-2 \text{J}^2 + \text{Ja})^4 \text{Cos}[4k] + \\
& 12 \text{i} (-16 \text{JdB} (\text{JdB} - \text{JdC}) \text{JdC} (-2 \text{J}^2 + \text{Ja} + 3 (\text{JdB} + \text{JdC})) - \\
& \quad 8 (-3 \text{Ja} (-2 \text{J}^2 + \text{Ja} - 2 \text{JdB}) \text{JdB} + \\
& \quad (4 \text{J}^2 - 10 \text{Ja} - 9 \text{JdB}) \text{JdB JdC} + 2 (\text{J}^2 + 5 \text{Ja}) \text{JdC}^2 + 3 \text{JdC}^3) \text{JpA} + \\
& 4 (-3 \text{Ja} (\text{Ja} - 4 \text{JdB}) - (9 \text{Ja} + \text{JdB}) \text{JdC} + 2 \text{J}^2 (3 \text{Ja} + \text{JdC})) \text{JpA}^2 + \\
& 2 (-6 \text{Ja} + 11 \text{JdC}) \text{JpA}^3 + \\
& (8 (\text{JdB}^2 (2 \text{J}^2 + 10 \text{Ja} + 3 \text{JdB}) + (6 \text{J}^2 \text{Ja} - 3 \text{Ja}^2 + 4 \text{J}^2 \text{JdB} - 10 \text{Ja JdB}) \text{JdC} + \\
& \quad 3 (2 \text{Ja} - 3 \text{JdB}) \text{JdC}^2) - 4 (\text{JdB} - \text{JdC}) (26 \text{J}^2 + 17 \text{Ja} + 3 (\text{JdB} + \text{JdC})) \\
& \quad \text{JpA} + 2 (24 \text{J}^2 + 7 \text{Ja} - 11 \text{JdB}) \text{JpA}^2 - 5 \text{JpA}^3) \text{JpB} - \\
& 2 (-6 \text{Ja}^2 - 18 \text{Ja JdB} + 24 \text{Ja JdC} - 2 \text{JdB JdC} + 7 \text{Ja JpA} - 11 \text{JdC JpA} + \\
& \quad 4 \text{J}^2 (3 \text{Ja} + \text{JdB} + 6 \text{JpA})) \text{JpB}^2 + (12 \text{Ja} - 22 \text{JdB} + 5 \text{JpA}) \text{JpB}^3) \\
& \text{Sin}[k] + 24 \text{i} (2 \text{JdC} (4 (2 \text{J}^2 - \text{Ja}) \text{JdB} (\text{JdB} - \text{JdC}) + \\
& \quad (\text{J}^2 (-6 \text{Ja} + 4 \text{JdC}) + \text{Ja} (3 \text{Ja} - 2 (3 \text{JdB} + \text{JdC}))) \text{JpA} + (4 \text{J}^2 + \text{Ja}) \text{JpA}^2) + \\
& (2 \text{JdB} ((-2 \text{J}^2 + \text{Ja}) (-3 \text{Ja} + 2 \text{JdB}) + 6 \text{Ja JdC}) + 6 \text{Ja} (\text{JdB} - \text{JdC}) \text{JpA} - \\
& \quad (4 \text{J}^2 + \text{Ja}) \text{JpA}^2) \text{JpB} - (4 \text{J}^2 + \text{Ja}) (2 \text{JdB} - \text{JpA}) \text{JpB}^2) \text{Sin}[2k]
\end{aligned}$$

$$\text{W12o4}[k_, \text{Ja}_-, \text{J}^2_-, \text{JdB}_-, \text{JpA}_-, \text{JpB}_-, \text{JdC}_-] := \frac{1}{1536}$$

$$\begin{aligned}
& (6 \text{JdC} (-8 \text{JdB}^2 (4 \text{JdB} + \text{JdC}) + 8 \text{JdB} (2 \text{JdB} + \text{JdC}) \text{JpA} - 2 (5 \text{JdB} + \text{JdC}) \text{JpA}^2 - 11 \text{JpA}^3) + \\
& 6 (16 \text{JdB}^3 + 14 \text{JdB}^2 \text{JpA} + 3 \text{JpA}^2 (\text{JdC} + \text{JpA}) - \text{JdB JpA} (6 \text{JdC} + \text{JpA})) \text{JpB} - \\
& 3 (24 \text{JdB}^2 + 64 \text{JdC}^2 - 54 \text{JdB JpA} + 17 \text{JpA}^2) \text{JpB}^2 + 48 \text{JpB}^4 + \\
& 24 \text{J}^3 (6 \text{JdB} - 8 \text{JdC} - 3 \text{JpA} + 4 \text{JpB}) + \text{Ja}^3 (-10 \text{JdB} - 72 \text{JdC} + 19 \text{JpA} + 36 \text{JpB}) -
\end{aligned}$$

$$\begin{aligned}
& Ja^2 (124 JdB^2 + 328 JdC^2 + 31 JpA^2 + 4 JdC (33 JpA - 64 JpB) - \\
& \quad 4 JdB (8 JdC + 35 JpA - 26 JpB) - 60 JpA JpB + 66 JpB^2) - \\
& 4 J2^2 (36 (JdB^2 - 2 JdB JdC + 2 JdC^2) + 31 JpA^2 + 92 JpA JpB + 26 JpB^2 + \\
& \quad Ja (102 JdB - 24 JdC - 17 JpA + 12 JpB)) + \\
& Ja (-24 JdB^3 - 12 JdB^2 (4 JdC + JpA - 11 JpB) + \\
& \quad 2 JdB (-84 JdC^2 + 114 JdC JpA + 27 JpA^2 + 272 JdC JpB - 93 JpA JpB - 71 JpB^2) + \\
& \quad JpA (340 JdC^2 - 6 JdC JpA + 27 JpA^2 - 272 JdC JpB + 24 JpA JpB + 43 JpB^2)) + \\
& 2 J2 (3 (8 JdB (JdB^2 + 4 JdB JdC + 7 JdC^2) - 4 (11 JdB^2 + 2 JdB JdC + 7 JdC^2) JpA - \\
& \quad 2 (JdB + 2 JdC) JpA^2 - 5 JpA^3) + \\
& \quad 2 (12 JdB (JdB - 9 JdC) - 2 (24 JdB + 37 JdC) JpA - 9 JpA^2) JpB + \\
& \quad (98 JdB + 19 JpA) JpB^2 + Ja^2 (-2 JdB - 120 JdC + 21 JpA + 60 JpB) + Ja (144 JdC^2 + \\
& \quad 212 JdC JpA + 70 JpA^2 - 4 JdB (18 JdC + JpA - 52 JpB) - 20 JpA JpB + 52 JpB^2)) + \\
& (-48 JdB JdC^2 (JdB + 2 JdC) + 48 JdC^3 JpA - 4 (48 JdB^2 + 19 JdC^2) JpA^2 + 48 JpA^4 + \\
& \quad 144 J2^3 (2 JdC - JpB) + 8 JdC (6 JdB (JdB + JdC) - (JdB - 12 JdC) JpA + 19 JpA^2) JpB + \\
& \quad (-28 JdB^2 + (36 JdC - 49 JpA) JpA + 20 JdB (-6 JdC + JpA)) JpB^2 - \\
& \quad 36 JdB JpB^3 + 2 Ja^3 (-8 JdB - 10 JdC + 6 JpA + 5 JpB) - \\
& \quad 2 Ja^2 (160 JdB^2 + 124 JdC^2 + 45 JpA^2 - 2 JdB (12 JdC + 70 JpA - 35 JpB) + 32 JdC \\
& \quad (4 JpA - 5 JpB) - 34 JpA JpB + 53 JpB^2) + 2 J2 (-4 Ja^2 (44 JdB + JdC - 20 JpA) + \\
& \quad 2 JdC (108 JdB^2 + 72 JdB JdC + 24 JdC^2 - 132 JdB JpA + 35 JpA^2) + \\
& \quad 8 Ja (12 JdB^2 - JdB (21 JdC + JpA) + JpA (50 JdC + 11 JpA)) + (2 (Ja^2 + 106 Ja \\
& \quad JdB - 6 (9 JdB^2 + 6 JdB JdC + 22 JdC^2)) + 4 (11 Ja - 29 JdB - 34 JdC) JpA + \\
& \quad 29 JpA^2) JpB + 4 (40 Ja - 4 JdB - 3 JdC + 4 JpA) JpB^2 - 30 JpB^3) + \\
& Ja (-2 JdC (108 JdB^2 + 24 JdC^2 - 4 (69 JdB + 28 JdC) JpA + 47 JpA^2) + \\
& \quad (4 (99 JdB^2 + 62 JdB JdC + 66 JdC^2) - 4 (79 JdB + 62 JdC) JpA + 31 JpA^2) JpB + \\
& \quad 12 (-JdB + JdC + 2 JpA) JpB^2 + 30 JpB^3) - \\
& 8 J2^2 (24 JdB^2 + 36 JdC^2 + 12 JdC JpA + 21 JpA^2 + Ja (102 JdC - 2 JpA - 51 JpB) + \\
& \quad 86 JpA JpB + 31 JpB^2 - 12 JdB (5 JdC + JpB))) Cos[k] - \\
& (48 J2^3 (2 JdB - 8 JdC - JpA + 4 JpB) + 4 Ja^3 (-5 JdB - 28 JdC + 6 JpA + 14 JpB) + \\
& \quad Ja^2 (124 JdB^2 - 16 JdC^2 + 8 JdC JpA + 75 JpA^2 - \\
& \quad 4 JdB (4 JdC + 45 JpA - 38 JpB) - 8 (4 JdC + JpA) JpB + 40 JpB^2) + 4 J2^2 \\
& \quad (36 JdB^2 - 48 JdC^2 - 24 JdC JpA + 31 JpA^2 + 4 Ja (3 JdB + 12 JdC - 10 JpA - 6 JpB) + \\
& \quad 80 JpA JpB + 32 JpB^2 + 24 JdB (-2 JdC + JpB)) + \\
& 2 (24 JdB^3 (-2 JdC + JpB) + JdB JpA (30 JdC JpA - 7 (2 JdC + 3 JpA) JpB + 5 JpB^2) + \\
& \quad 2 JdB^2 (12 JdC JpA + JpB (-3 JpA + JpB)) - \\
& \quad JpA^2 (-8 JdC^2 + JpB (-9 JpA + JpB) + JdC (15 JpA + JpB))) + 2 J2 (-24 JdB^3 + \\
& \quad 2 Ja^2 (46 JdB + 56 JdC - 13 JpA - 28 JpB) + 12 JdB^2 (-4 JdC + 11 JpA + 2 JpB) + \\
& \quad 2 Ja (48 JdB JdC + 48 JdC^2 - 2 JdB JpA - 45 JpA^2 - 32 (3 JdB + JpA) JpB - 32 JpB^2) + \\
& \quad JdB (72 JdC^2 + 48 JdC JpA + 6 JpA^2 - 72 JdC JpB + 40 JpA JpB + 58 JpB^2) + \\
& \quad JpA (-36 JdC^2 + 15 JpA^2 - 34 JpA JpB - 25 JpB^2 + 4 JdC (JpA + 7 JpB))) + \\
& Ja (24 JdB^3 + JpA (4 JdC^2 + 6 JdC JpA - 3 JpA^2 - 16 JdC JpB + 27 JpB^2) - \\
& \quad 4 JdB^2 (12 JdC + 23 (3 JpA + JpB)) + \\
& \quad JdB (-72 JdC^2 + 42 JpA^2 + 62 JpA JpB - 78 JpB^2 + 4 JdC (-5 JpA + 28 JpB)))) \\
& Cos[2 k] + (-4 J2 (2 Ja^2 (14 JdB + 45 JdC - 9 JpA) + 15 JdC (-2 JdB + JpA)^2 + \\
& \quad 2 Ja (12 JdB^2 - 2 JdB JpA - 7 JpA^2)) + \\
& 8 J2^2 (12 JdB^2 - 8 JpA^2 + Ja (-12 JdB + 90 JdC + 4 JpA - 45 JpB)) +
\end{aligned}$$

$$\begin{aligned}
& \text{Ja} \left( 8 \text{Ja} (\text{JdB} - \text{JpA}) (\text{JdB} + 2 \text{JpA}) + \text{Ja}^2 (56 \text{JdB} + 60 \text{JdC} - 32 \text{JpA} - 30 \text{JpB}) + \right. \\
& \quad \left. 15 (-2 \text{JdB} + \text{JpA})^2 (2 \text{JdC} - \text{JpB}) \right) + \\
& 30 \text{J2} \left( 6 \text{Ja}^2 + (-2 \text{JdB} + \text{JpA})^2 \right) \text{JpB} + 48 \text{J2}^3 (4 \text{JdB} - 2 (5 \text{JdC} + \text{JpA}) + 5 \text{JpB}) \\
& \text{Cos}[3 \text{k}] - 15 (2 \text{J2} - \text{Ja})^3 (2 \text{JdB} - \text{JpA}) \text{Cos}[4 \text{k}] + \\
& \text{i} \left( 8 \text{JdB} (16 \text{Ja}^3 + \text{Ja}^2 (42 \text{JdB} - 2 \text{JdC}) + 3 \text{Ja} \text{JdC} (5 \text{JdB} + 4 \text{JdC}) + 6 \text{JdC}^2 (\text{JdB} + 6 \text{JdC})) + \right. \\
& \quad 192 \text{J2}^3 (2 \text{JdB} - \text{JpA}) - \\
& \quad 4 (15 \text{Ja}^3 + 36 \text{JdC}^3 + 2 \text{Ja} \text{JdC} (67 \text{JdB} + 5 \text{JdC}) + 2 \text{Ja}^2 (29 \text{JdB} + 6 \text{JdC})) \text{JpA} + \\
& \quad 2 (21 \text{Ja}^2 + 96 \text{JdB}^2 + 95 \text{Ja} \text{JdC} + 34 \text{JdC}^2) \text{JpA}^2 - 48 \text{JpA}^4 + \\
& \quad 4 \text{J2} (4 \text{Ja}^2 (8 \text{JdB} - 5 \text{JpA}) - 3 \text{JdC} (20 \text{JdB}^2 + 8 \text{JdB} \text{JdC} - 28 \text{JdB} \text{JpA} + 8 \text{JdC} \text{JpA} + \\
& \quad \quad 21 \text{JpA}^2) - 4 \text{Ja} (24 \text{JdB}^2 + 2 \text{JpA} (\text{JdC} + \text{JpA}) + \text{JdB} (3 \text{JdC} + \text{JpA})) - 2 \text{J2} \\
& \quad (4 (10 \text{Ja}^2 + 53 \text{Ja} \text{JdB} - 15 \text{JdB}^2 - 2 \text{Ja} \text{JdC} + 6 \text{JdB} \text{JdC}) - 4 (21 \text{Ja} + 45 \text{JdB} + 14 \text{JdC}) \\
& \quad \quad \text{JpA} + 9 \text{JpA}^2) \text{JpB} - (28 \text{Ja}^3 - 4 \text{Ja}^2 (31 \text{JdB} + 10 \text{JdC} - 13 \text{JpA}) + \\
& \quad 4 \text{JdC} (12 \text{JdB} (\text{JdB} + 3 \text{JdC}) + 2 (-8 \text{JdB} + 9 \text{JdC}) \text{JpA} + 43 \text{JpA}^2) + \\
& \quad \text{Ja} (4 (71 \text{JdB}^2 + 52 \text{JdB} \text{JdC} - 72 \text{JdC}^2) - 4 (57 \text{JdB} + 31 \text{JdC}) \text{JpA} + 55 \text{JpA}^2)) \text{JpB} + \\
& \quad 8 \text{J2} (5 \text{Ja} + 2 \text{JdB} + 13 \text{JpA}) \text{JpB}^2 - (44 \text{Ja}^2 + 4 \text{JdB}^2 + 16 (\text{JdB} - 3 \text{JdC}) \text{JpA} - \\
& \quad \quad 53 \text{JpA}^2 + 24 \text{Ja} (4 \text{JdC} + \text{JpA})) \text{JpB}^2 - 12 (2 \text{Ja} - 8 \text{JdB} + 3 \text{JpA}) \text{JpB}^3 + \\
& \quad 8 \text{J2}^2 (48 \text{JdB}^2 + 12 \text{JdB} (-\text{JdC} + \text{JpB}) + \text{JpA} (-12 \text{JdC} + 5 \text{JpA} + 6 \text{JpB}) + \\
& \quad \quad \text{Ja} (-24 \text{JdB} + 14 \text{JpA} + 34 \text{JpB})) \text{Sin}[k] - \text{i} (192 \text{J2}^3 (2 \text{JdB} - \text{JpA}) - \\
& \quad 2 \text{JdC} (-48 \text{JdB}^3 + 24 \text{JdB}^2 \text{JpA} + 30 \text{JdB} \text{JpA}^2 + (8 \text{JdC} - 15 \text{JpA}) \text{JpA}^2) + \\
& \quad 2 (-24 \text{JdB}^3 + 6 \text{JdB}^2 \text{JpA} + (\text{JdC} - 9 \text{JpA}) \text{JpA}^2 + 7 \text{JdB} \text{JpA} (2 \text{JdC} + 3 \text{JpA})) \text{JpB} + \\
& \quad 2 (-2 \text{JdB}^2 - 5 \text{JdB} \text{JpA} + \text{JpA}^2) \text{JpB}^2 + \text{Ja}^3 (-40 \text{JdB} + 6 \text{JpA} + 8 \text{JpB}) + \\
& \quad \text{Ja}^2 (-124 \text{JdB}^2 - \text{JpA} (8 \text{JdC} + 75 \text{JpA}) + 4 \text{JdB} (4 \text{JdC} + 45 \text{JpA} - 38 \text{JpB}) + \\
& \quad \quad 8 (2 \text{JdC} + \text{JpA}) \text{JpB} - 8 \text{JpB}^2) - 4 \text{J2}^2 (36 \text{JdB}^2 + 2 \text{Ja} (96 \text{JdB} - 65 \text{JpA} - 4 \text{JpB}) + \\
& \quad \quad 24 \text{JdB} (-2 \text{JdC} + \text{JpB}) + \text{JpA} (-24 \text{JdC} + 31 \text{JpA} + 80 \text{JpB})) + \\
& \quad 2 \text{J2} (24 \text{JdB}^3 + 12 \text{JdB}^2 (4 \text{JdC} - 11 \text{JpA} - 2 \text{JpB}) - \text{JpA} (84 \text{JdC}^2 + 15 \text{JpA}^2 + \\
& \quad \quad 4 \text{JdC} (\text{JpA} - 23 \text{JpB}) - 34 \text{JpA} \text{JpB} + 5 \text{JpB}^2) + 8 \text{Ja}^2 (11 \text{JdB} - 2 (4 \text{JpA} + \text{JpB})) + \\
& \quad 2 \text{JdB} (84 \text{JdC}^2 - 3 \text{JpA}^2 - 20 \text{JpA} \text{JpB} + \text{JpB}^2 - 12 \text{JdC} (2 \text{JpA} + 7 \text{JpB})) + 2 \text{Ja} \\
& \quad (45 \text{JpA}^2 + 32 \text{JpA} \text{JpB} + 4 \text{JpB} (-2 \text{JdC} + \text{JpB}) + 2 \text{JdB} (-24 \text{JdC} + \text{JpA} + 48 \text{JpB})) + \\
& \quad \text{Ja} (-24 \text{JdB}^3 + 2 \text{JdB} (-84 \text{JdC}^2 + 10 \text{JdC} \text{JpA} - 21 \text{JpA}^2 + 64 \text{JdC} \text{JpB} - \\
& \quad \quad 31 \text{JpA} \text{JpB} + 9 \text{JpB}^2) + 4 \text{JdB}^2 (12 \text{JdC} + 23 (3 \text{JpA} + \text{JpB})) + \\
& \quad \text{JpA} (116 \text{JdC}^2 - 2 \text{JdC} (3 \text{JpA} + 52 \text{JpB}) + 3 (\text{JpA}^2 + \text{JpB}^2))) \text{Sin}[2 \text{k}] - \\
& \text{i} (96 \text{J2}^3 (2 \text{JdB} - \text{JpA}) + 32 \text{J2}^2 (3 \text{JdB} (-\text{Ja} + \text{JdB}) + \text{Ja} \text{JpA} - 2 \text{JpA}^2) + \\
& \quad 4 \text{J2} (-15 \text{JdC} (-2 \text{JdB} + \text{JpA})^2 + \text{Ja}^2 (-28 \text{JdB} + 18 \text{JpA}) + \\
& \quad \quad \text{Ja} (-24 \text{JdB}^2 + 4 \text{JdB} \text{JpA} + 14 \text{JpA}^2)) + \text{Ja} (8 \text{Ja}^2 (7 \text{JdB} - 4 \text{JpA}) + \\
& \quad \quad 8 \text{Ja} (\text{JdB} - \text{JpA}) (\text{JdB} + 2 \text{JpA}) + 15 (-2 \text{JdB} + \text{JpA})^2 (2 \text{JdC} - \text{JpB})) + \\
& \quad 30 \text{J2} (-2 \text{JdB} + \text{JpA})^2 \text{JpB} \text{Sin}[3 \text{k}] + 15 \text{i} (2 \text{J2} - \text{Ja})^3 (2 \text{JdB} - \text{JpA}) \text{Sin}[4 \text{k}]
\end{aligned}$$

(\* FIFTH ORDER \*)

(\* The results of the fifth-order expressions W11o5,

W22o5=Conjugate[W11o5], W12o5 and W21o5=Conjugate[W12o5] are \*)

W11o5[k\_, Ja\_, J2\_, JdB\_, JpA\_, JpB\_, JdC\_] :=

$$\frac{1}{73728} \left( -46080 \text{J2}^5 + 70272 \text{J2}^4 \text{Ja} - 864 \text{Ja}^5 - \right.$$

$$\begin{aligned}
& 16 J_2^3 (3564 J_a^2 - 612 J_{dB}^2 - 612 J_{dC}^2 - 810 J_{dC} J_{pA} + 431 J_{pA}^2 + \\
& \quad 18 J_{dB} (50 J_{dC} + 74 J_{pA} - 45 J_{pB}) + 1332 J_{dC} J_{pB} + 1609 J_{pA} J_{pB} + 431 J_{pB}^2) + \\
& 2 J_a (2 J_{dC} (-504 J_{dB} (15 J_{dB}^2 - 4 J_{dB} J_{dC} + 15 J_{dC}^2) + 4 (5339 J_{dB}^2 + \\
& \quad 396 J_{dB} J_{dC} + 1421 J_{dC}^2) J_{pA} - 18 (671 J_{dB} + 26 J_{dC}) J_{pA}^2 + 709 J_{pA}^3) + \\
& \quad (8 J_{dB} (1421 J_{dB}^2 + 396 J_{dB} J_{dC} + 5339 J_{dC}^2) - 4 (4447 J_{dB}^2 + 1080 J_{dB} J_{dC} + \\
& \quad 4447 J_{dC}^2) J_{pA} + 2 (3691 J_{dB} - 216 J_{dC}) J_{pA}^2 - 953 J_{pA}^3) J_{pB} - \\
& \quad 2 (468 J_{dB}^2 + 18 J_{dB} (671 J_{dC} + 12 J_{pA}) - J_{pA} (3691 J_{dC} + 126 J_{pA})) J_{pB}^2 + \\
& \quad (1418 J_{dB} - 953 J_{pA}) J_{pB}^3) + \\
& 9 (-160 (3 J_{dB}^5 + 13 J_{dB}^3 J_{dC}^2 + 13 J_{dB}^2 J_{dC}^3 + 3 J_{dC}^5) + \\
& \quad 16 J_{dB} (93 J_{dB}^3 + 61 J_{dB} J_{dC}^2 + 90 J_{dC}^3) J_{pA} - \\
& \quad 8 (206 J_{dB}^3 + 75 J_{dB} J_{dC}^2 + 25 J_{dC}^3) J_{pA}^2 - 4 (78 J_{dB}^2 + 89 J_{dC}^2) J_{pA}^3 + 954 J_{dB} J_{pA}^4 - \\
& \quad 15 J_{pA}^5 + 4 J_{dC} (4 (90 J_{dB}^3 + 61 J_{dB}^2 J_{dC} + 93 J_{dC}^3) - 180 J_{dB} (J_{dB} + J_{dC}) J_{pA} + \\
& \quad (574 J_{dB} + 29 J_{dC}) J_{pA}^2 - 79 J_{pA}^3) J_{pB} - (8 (25 J_{dB}^3 + 75 J_{dB}^2 J_{dC} + 206 J_{dC}^3) - \\
& \quad 4 J_{dB} (29 J_{dB} + 574 J_{dC}) J_{pA} + 502 (J_{dB} + J_{dC}) J_{pA}^2 + 33 J_{pA}^3) J_{pB}^2 - \\
& \quad (356 J_{dB}^2 + 312 J_{dC}^2 + 316 J_{dB} J_{pA} + 33 J_{pA}^2) J_{pB}^3 + 954 J_{dC} J_{pB}^4 - 15 J_{pB}^5) + \\
& 2 J_a^3 (4516 J_{dB}^2 + 4516 J_{dC}^2 + 446 J_{dC} J_{pA} + 345 J_{pA}^2 - 4084 J_{dC} J_{pB} + \\
& \quad 917 J_{pA} J_{pB} + 345 J_{pB}^2 + J_{dB} (2388 J_{dC} - 4084 J_{pA} + 446 J_{pB})) - \\
& 2 J_a^2 (3448 J_{dB}^3 + 3448 J_{dC}^3 + J_{dC}^2 (548 J_{pA} - 9132 J_{pB}) - \\
& \quad 4 J_{dB}^2 (658 J_{dC} + 2283 J_{pA} - 137 J_{pB}) - (J_{pA} + J_{pB}) \\
& \quad (345 J_{pA}^2 + 1612 J_{pA} J_{pB} + 345 J_{pB}^2) + 2 J_{dC} (841 J_{pA}^2 + 1330 J_{pA} J_{pB} + 3997 J_{pB}^2) + \\
& \quad J_{dB} (-2632 J_{dC}^2 + 7994 J_{pA}^2 + 2660 J_{pA} J_{pB} + 1682 J_{pB}^2 + 3224 J_{dC} (J_{pA} + J_{pB}))) + \\
& 8 J_2^2 (3924 J_a^3 + 1224 J_{dB}^3 + 1656 J_{dB}^2 J_{dC} + 1656 J_{dB} J_{dC}^2 + 1224 J_{dC}^3 - 756 J_{dB}^2 J_{pA} - \\
& \quad 2952 J_{dB} J_{dC} J_{pA} + 2196 J_{dC}^2 J_{pA} - 5210 J_{dB} J_{pA}^2 + 658 J_{dC} J_{pA}^2 + 1129 J_{pA}^3 + \\
& \quad (36 (61 J_{dB}^2 - 82 J_{dB} J_{dC} - 21 J_{dC}^2) - 3900 (J_{dB} + J_{dC}) J_{pA} + 415 J_{pA}^2) J_{pB} + \\
& \quad (658 J_{dB} - 5210 J_{dC} + 415 J_{pA}) J_{pB}^2 + 1129 J_{pB}^3 + \\
& \quad J_a (-756 J_{dB}^2 - 756 J_{dC}^2 + 2594 J_{dC} J_{pA} + 2283 J_{pA}^2 + 1476 J_{dC} J_{pB} + \\
& \quad 1603 J_{pA} J_{pB} + 2283 J_{pB}^2 + 2 J_{dB} (918 J_{dC} + 738 J_{pA} + 1297 J_{pB}))) + \\
& 4 J_2 (612 J_a^4 + 2 J_{dC} (360 J_{dB} (25 J_{dB}^2 + 2 J_{dB} J_{dC} + 25 J_{dC}^2) - 108 (173 J_{dB}^2 + \\
& \quad 12 J_{dB} J_{dC} + 35 J_{dC}^2) J_{pA} + 2 (4667 J_{dB} + 504 J_{dC}) J_{pA}^2 - 1409 J_{pA}^3) + \\
& \quad (-216 J_{dB} (35 J_{dB}^2 + 12 J_{dB} J_{dC} + 173 J_{dC}^2) + 4 (2819 J_{dB}^2 - 1800 J_{dB} J_{dC} + \\
& \quad 2819 J_{dC}^2) J_{pA} + 18 (-287 J_{dB} + 128 J_{dC}) J_{pA}^2 + 2221 J_{pA}^3) J_{pB} + \\
& \quad 2 (1008 J_{dB}^2 - 9 J_{pA} (287 J_{dC} + 71 J_{pA}) + 2 J_{dB} (4667 J_{dC} + 576 J_{pA})) J_{pB}^2 + \\
& \quad (-2818 J_{dB} + 2221 J_{pA}) J_{pB}^3 - \\
& \quad J_a^2 (10420 J_{dB}^2 + 10420 J_{dC}^2 + 3706 J_{dC} J_{pA} + 3997 J_{pA}^2 - 9988 J_{dC} J_{pB} + \\
& \quad 191 J_{pA} J_{pB} + 3997 J_{pB}^2 + J_{dB} (6780 J_{dC} - 9988 J_{pA} + 3706 J_{pB})) + \\
& \quad 2 J_a (-2664 J_{dB}^3 - 2664 J_{dC}^3 + 12 J_{dB}^2 (-246 J_{dC} + 123 J_{pA} + 79 J_{pB}) + \\
& \quad 12 J_{dC}^2 (79 J_{pA} + 123 J_{pB}) - (J_{pA} + J_{pB}) (1021 J_{pA}^2 - 224 J_{pA} J_{pB} + 1021 J_{pB}^2) + \\
& \quad J_{dC} (-806 J_{pA}^2 + 428 J_{pA} J_{pB} + 4994 J_{pB}^2) + \\
& \quad J_{dB} (-2952 J_{dC}^2 + 4994 J_{pA}^2 + 428 J_{pA} J_{pB} - 806 J_{pB}^2 + 8216 J_{dC} (J_{pA} + J_{pB})))) + \\
& 2 (- (7488 J_2^5 + 8352 J_2^4 J_a + 630 J_a^5 + 4 J_{dC} (-72 J_{dB} (J_{dB} + J_{dC}) (14 J_{dB}^2 - 15 J_{dB} \\
& \quad J_{dC} + 14 J_{dC}^2) + 36 (44 J_{dB}^3 + 25 J_{dB}^2 J_{dC} + 14 J_{dC}^3) J_{pA} + 2 (540 J_{dB}^2 - \\
& \quad 265 J_{dB} J_{dC} + 371 J_{dC}^2) J_{pA}^2 + (-180 J_{dB} + 31 J_{dC}) J_{pA}^3 - 315 J_{pA}^4) + \\
& \quad 2 (72 J_{dB} (14 J_{dB}^3 + 25 J_{dB} J_{dC}^2 + 44 J_{dC}^3) - 16 (J_{dB} + J_{dC}) \\
& \quad (162 J_{dB}^2 - 283 J_{dB} J_{dC} + 162 J_{dC}^2) J_{pA} - 2 (720 J_{dB}^2 + 264 J_{dB} J_{dC} + \\
& \quad 2305 J_{dC}^2) J_{pA}^2 + 4 (252 J_{dB} - 97 J_{dC}) J_{pA}^3 + 117 J_{pA}^4) J_{pB} +
\end{aligned}$$

$$\begin{aligned}
& (8 \text{ JdB} (371 \text{ JdB}^2 - 265 \text{ JdB JdC} + 540 \text{ JdC}^2) - 4 (2305 \text{ JdB}^2 + 264 \text{ JdB JdC} + \\
& \quad 720 \text{ JdC}^2) \text{ JpA} + 2810 (\text{JdB} + \text{JdC}) \text{ JpA}^2 + 49 \text{ JpA}^3) \text{ JpB}^2 + \\
& (124 \text{ JdB}^2 + 7 \text{ JpA} (288 \text{ JdC} + 7 \text{ JpA}) - 8 \text{ JdB} (90 \text{ JdC} + 97 \text{ JpA})) \text{ JpB}^3 + \\
& 18 (-70 \text{ JdB} + 13 \text{ JpA}) \text{ JpB}^4 + \\
& 8 \text{ J}2^3 (1044 \text{ Ja}^2 + 2484 \text{ JdB}^2 - 5904 \text{ JdB JdC} + 2484 \text{ JdC}^2 - 2052 \text{ JdB JpA} + \\
& \quad 2664 \text{ JdC JpA} + 2333 \text{ JpA}^2 + 36 (74 \text{ JdB} - 57 \text{ JdC} + 55 \text{ JpA}) \text{ JpB} + 2333 \text{ JpB}^2) - \\
& \text{Ja}^3 (5748 \text{ JdB}^2 + 5748 \text{ JdC}^2 + 4396 \text{ JdC JpA} + 2037 \text{ JpA}^2 - 4548 \text{ JdC JpB} - \\
& \quad 700 \text{ JpA JpB} + 2037 \text{ JpB}^2 + \text{JdB} (-6784 \text{ JdC} - 4548 \text{ JpA} + 4396 \text{ JpB})) + \\
& 2 \text{Ja}^2 (2808 \text{ JdB}^3 + 2808 \text{ JdC}^3 + 4 \text{JdC}^2 (326 \text{ JpA} - 1543 \text{ JpB}) + 4 \text{JdB}^2 (1100 \text{ JdC} - \\
& \quad 1543 \text{ JpA} + 326 \text{ JpB}) - (\text{JpA} + \text{JpB}) (469 \text{ JpA}^2 - 422 \text{ JpA JpB} + 469 \text{ JpB}^2) + \\
& \quad 2 \text{JdC} (755 \text{ JpA}^2 - 71 \text{ JpA JpB} + 1893 \text{ JpB}^2) + 2 \text{JdB} (2200 \text{ JdC}^2 + 1893 \text{ JpA}^2 - \\
& \quad 71 \text{ JpA JpB} + 755 \text{ JpB}^2 - 1186 \text{ JdC} (\text{JpA} + \text{JpB}))) + \text{Ja} (-432 \text{ JdB}^4 - \\
& \quad 432 \text{ JdC}^4 + 1485 \text{ JpA}^4 + 216 \text{ JdB}^3 (6 \text{ JdC} - 12 \text{ JpA} - 25 \text{ JpB}) + 1393 \text{ JpA}^3 \text{ JpB} - \\
& \quad 2093 \text{ JpA}^2 \text{ JpB}^2 + 1393 \text{ JpA JpB}^3 + 1485 \text{ JpB}^4 - 216 \text{ JdC}^3 (25 \text{ JpA} + 12 \text{ JpB}) - \\
& \quad 4 \text{JdC}^2 (853 \text{ JpA}^2 - 3291 \text{ JpA JpB} + 378 \text{ JpB}^2) - 4 \text{JdB}^2 (2772 \text{ JdC}^2 + \\
& \quad 3954 \text{ JdC JpA} + 378 \text{ JpA}^2 - 100 \text{ JdC JpB} - 3291 \text{ JpA JpB} + 853 \text{ JpB}^2) + 2 \text{JdC} \\
& \quad (1453 \text{ JpA}^3 + 2898 \text{ JpA}^2 \text{ JpB} - 2993 \text{ JpA JpB}^2 - 756 \text{ JpB}^3) + 2 \text{JdB} (648 \text{ JdC}^3 - \\
& \quad 756 \text{ JpA}^3 + 4 \text{JdC}^2 (50 \text{ JpA} - 1977 \text{ JpB}) - 2993 \text{ JpA}^2 \text{ JpB} + 2898 \text{ JpA JpB}^2 + \\
& \quad 1453 \text{ JpB}^3 + 6 \text{JdC} (401 \text{ JpA}^2 - 188 \text{ JpA JpB} + 401 \text{ JpB}^2))) + 2 \text{J}2 \\
& (894 \text{ Ja}^4 + 432 \text{ JdB}^4 + 432 \text{ JdC}^4 - 648 \text{ JdC}^3 \text{ JpA} + 3828 \text{ JdC}^2 \text{ JpA}^2 - 786 \text{ JdC JpA}^3 - \\
& \quad 1773 \text{ JpA}^4 + (2592 \text{ JdC}^3 + 4724 \text{ JdC}^2 \text{ JpA} - 8492 \text{ JdC JpA}^2 - 2361 \text{ JpA}^3) \text{ JpB} + \\
& \quad (360 \text{ JdC}^2 + 346 \text{ JdC JpA} + 2969 \text{ JpA}^2) \text{ JpB}^2 + 3 (888 \text{ JdC} - 787 \text{ JpA}) \text{ JpB}^3 - \\
& \quad 1773 \text{ JpB}^4 - 72 \text{ JdB}^3 (34 \text{ JdC} + 9 (-4 \text{ JpA} + \text{JpB})) + 4 \text{JdB}^2 \\
& \quad (2052 \text{ JdC}^2 + 90 \text{ JpA}^2 + 1181 \text{ JpA JpB} + 957 \text{ JpB}^2 - 54 \text{ JdC} (\text{JpA} + 42 \text{ JpB})) + \\
& \quad \text{Ja}^2 (13996 \text{ JdB}^2 + 13996 \text{ JdC}^2 + 12032 \text{ JdC JpA} + 7491 \text{ JpA}^2 - 4 (2983 \text{ JdC} + \\
& \quad 842 \text{ JpA}) \text{ JpB} + 7491 \text{ JpB}^2 + 4 \text{JdB} (952 \text{ JdC} - 2983 \text{ JpA} + 3008 \text{ JpB})) + \\
& \quad 2 \text{JdB} (-1224 \text{ JdC}^3 + 1332 \text{ JpA}^3 + 173 \text{ JpA}^2 \text{ JpB} - 4246 \text{ JpA JpB}^2 - 393 \text{ JpB}^3 - \\
& \quad 108 \text{ JdC}^2 (42 \text{ JpA} + \text{JpB}) + 2 \text{JdC} (461 \text{ JpA}^2 + 5676 \text{ JpA JpB} + 461 \text{ JpB}^2)) + \\
& \quad 2 \text{Ja} (-6544 \text{ JdC}^2 \text{ JpA} + 16 \text{ JdB}^2 (261 \text{ JdC} - 409 \text{ JpB}) + (\text{JpA} + \text{JpB}) \\
& \quad (816 \text{ JpA}^2 - 359 \text{ JpA JpB} + 816 \text{ JpB}^2) - 2 \text{JdC} (659 \text{ JpA}^2 - 741 \text{ JpA JpB} + \\
& \quad 2288 \text{ JpB}^2) + 2 \text{JdB} (2088 \text{ JdC}^2 - 2288 \text{ JpA}^2 + 741 \text{ JpA JpB} - \\
& \quad 659 \text{ JpB}^2 - 3130 \text{ JdC} (\text{JpA} + \text{JpB}))) + 4 \text{J}2^2 (-6636 \text{ Ja}^3 - \\
& \quad \text{Ja} (5292 \text{ JdB}^2 - 6480 \text{ JdB JdC} + 5292 \text{ JdC}^2 - 3996 \text{ JdB JpA} + 11252 \text{ JdC} \\
& \quad \text{JpA} + 6427 \text{ JpA}^2 + 4 (2813 \text{ JdB} - 999 \text{ JdC} + 288 \text{ JpA}) \text{ JpB} + 6427 \text{ JpB}^2) + \\
& \quad 2 (936 \text{ JdB}^3 + 936 \text{ JdC}^3 - 36 \text{ JdB}^2 (62 \text{ JdC} + 13 \text{ JpA} - 21 \text{ JpB}) + 36 \text{ JdC}^2 \\
& \quad (21 \text{ JpA} - 13 \text{ JpB}) - 9 (\text{JpA} + \text{JpB}) (27 \text{ JpA}^2 + 38 \text{ JpA JpB} + 27 \text{ JpB}^2) + \\
& \quad 2 \text{JdC} (573 \text{ JpA}^2 + 1340 \text{ JpA JpB} + 979 \text{ JpB}^2) + 2 \text{JdB} (-1116 \text{ JdC}^2 + 979 \\
& \quad \text{JpA}^2 + 1340 \text{ JpA JpB} + 573 \text{ JpB}^2 + 180 \text{ JdC} (\text{JpA} + \text{JpB})))) \text{Cos}[k] + \\
& (7488 \text{ J}2^5 - 23904 \text{ J}2^4 \text{ Ja} - 566 \text{ Ja}^5 - 8 \text{JdC}^2 (216 \text{ JdB}^2 (\text{JdB} + \text{JdC}) - \\
& \quad 108 \text{ JdB} (\text{JdB} + 2 \text{JdC}) \text{ JpA} + 2 (-25 \text{ JdB} + 23 \text{JdC}) \text{ JpA}^2 + 25 \text{JpA}^3) + \\
& \quad 8 \text{JdC} (108 \text{ JdB}^2 (2 \text{JdB} + \text{JdC}) - 32 \text{JdB} (\text{JdB} + \text{JdC}) \text{ JpA} - \\
& \quad (126 \text{ JdB} + 23 \text{JdC}) \text{ JpA}^2 + 44 \text{JpA}^3) \text{ JpB} - 2 (8 \text{JdB}^2 (23 \text{JdB} - 25 \text{JdC}) + \\
& \quad 4 \text{JdB} (23 \text{JdB} + 126 \text{JdC}) \text{ JpA} - 226 (\text{JdB} + \text{JdC}) \text{ JpA}^2 + 67 \text{JpA}^3) \\
& \quad \text{JpB}^2 - 2 (100 \text{ JdB}^2 - 176 \text{JdB JpA} + 67 \text{JpA}^2) \text{ JpB}^3 + \text{Ja}^3 \\
& \quad (2 (720 \text{ JdB}^2 + 720 \text{ JdC}^2 + 775 \text{ JdC JpA} + 524 \text{ JpA}^2 - 2 \text{JdB} (539 \text{ JdC} + 360 \text{ JpA})) +
\end{aligned}$$

$$\begin{aligned}
& 5 (310 \text{ JdB} - 9 (32 \text{ JdC} + 23 \text{ JpA})) \text{ JpB} + 1048 \text{ JpB}^2) - 8 \text{ J}^2 (964 \text{ Ja}^2 - 1530 \\
& \text{ JdC JpA} + 1376 \text{ JpA}^2 + 1530 \text{ JdB} (2 \text{ JdC} - \text{ JpB}) + 3037 \text{ JpA JpB} + 1376 \text{ JpB}^2) + \\
& 4 \text{ J}^2 (36 (191 \text{ Ja}^3 + 371 \text{ Ja JdB JdC} - 4 (\text{ JdB} + \text{ JdC}) (\text{ JdB}^2 + 3 \text{ JdB JdC} + \text{ JdC}^2)) + \\
& 6 (-337 \text{ Ja JdC} + 12 (\text{ JdB}^2 + 16 \text{ JdB JdC} - 12 \text{ JdC}^2)) \text{ JpA} + 4 (1016 \text{ Ja} - \\
& 183 \text{ JdB} - 468 \text{ JdC}) \text{ JpA}^2 - 290 \text{ JpA}^3 + (\text{ Ja} (-2022 \text{ JdB} + 4571 \text{ JpA}) + \\
& 8 (9 (-12 \text{ JdB}^2 + 16 \text{ JdB JdC} + \text{ JdC}^2) - 194 (\text{ JdB} + \text{ JdC}) \text{ JpA} + 81 \text{ JpA}^2)) \\
& \text{ JpB} + 4 (1016 \text{ Ja} - 468 \text{ JdB} - 183 \text{ JdC} + 162 \text{ JpA}) \text{ JpB}^2 - 290 \text{ JpB}^3) + \\
& 2 \text{ J}^2 (-2790 \text{ Ja}^4 + 4 \text{ JdC} (-36 \text{ JdB} (20 \text{ JdB}^2 + 3 \text{ JdB JdC} + 20 \text{ JdC}^2) + \\
& 72 (23 \text{ JdB}^2 + 3 \text{ JdB JdC} + 5 \text{ JdC}^2)) \text{ JpA} - 3 (404 \text{ JdB} + 19 \text{ JdC}) \text{ JpA}^2 - \\
& 46 \text{ JpA}^3) + 8 (36 \text{ JdB} (5 \text{ JdB}^2 + 3 \text{ JdB JdC} + 23 \text{ JdC}^2) - 12 (24 \text{ JdB}^2 + \\
& 43 \text{ JdB JdC} + 24 \text{ JdC}^2)) \text{ JpA} + (241 \text{ JdB} + 242 \text{ JdC}) \text{ JpA}^2 + 11 \text{ JpA}^3) \text{ JpB} + \\
& (-12 \text{ JdB} (19 \text{ JdB} + 404 \text{ JdC}) + 8 (242 \text{ JdB} + 241 \text{ JdC}) \text{ JpA} - 295 \text{ JpA}^2) \text{ JpB}^2 + \\
& 8 (-23 \text{ JdB} + 11 \text{ JpA}) \text{ JpB}^3 - \text{ Ja}^2 (1184 \text{ JdB}^2 + 1184 \text{ JdC}^2 - 694 \text{ JdC JpA} + \\
& 3672 \text{ JpA}^2 + 2 \text{ JdB} (8006 \text{ JdC} - 592 \text{ JpA} - 347 \text{ JpB}) - 1184 \text{ JdC JpB} + 283 \\
& \text{ JpA JpB} + 3672 \text{ JpB}^2) + 2 \text{ Ja} (144 (\text{ JdB} + \text{ JdC}) (\text{ JdB}^2 + 7 \text{ JdB JdC} + \text{ JdC}^2) + \\
& 4 (-18 \text{ JdB}^2 + 422 \text{ JdB JdC} + 627 \text{ JdC}^2)) \text{ JpA} + 4 (183 \text{ JdB} + 329 \text{ JdC}) \text{ JpA}^2 + \\
& 290 \text{ JpA}^3 + (4 (627 \text{ JdB}^2 + 422 \text{ JdB JdC} - 18 \text{ JdC}^2) - 1644 (\text{ JdB} + \text{ JdC}) \text{ JpA} - \\
& 373 \text{ JpA}^2) \text{ JpB} + (1316 \text{ JdB} + 732 \text{ JdC} - 373 \text{ JpA}) \text{ JpB}^2 + 290 \text{ JpB}^3) + \\
& 2 \text{ Ja}^2 (536 \text{ JdB}^3 + 536 \text{ JdC}^3 - 4 \text{ JdC}^2 (126 \text{ JpA} + 83 \text{ JpB}) - 4 \text{ JdB}^2 \\
& (1034 \text{ JdC} + 83 \text{ JpA} + 126 \text{ JpB}) - 5 (\text{ JpA} + \text{ JpB}) (17 \text{ JpA}^2 + \text{ JpA JpB} + 17 \text{ JpB}^2) - \\
& 2 \text{ JdC} (25 \text{ JpA}^2 - 512 \text{ JpA JpB} + 227 \text{ JpB}^2) + \\
& \text{ JdB} (-4136 \text{ JdC}^2 - 454 \text{ JpA}^2 + 1024 \text{ JpA JpB} - 50 \text{ JpB}^2 + 488 \text{ JdC} (\text{ JpA} + \text{ JpB}))) + \\
& \text{ Ja} (32 \text{ JdB}^3 (90 \text{ JdC} - 83 \text{ JpB}) - 4 \text{ JdB}^2 (324 \text{ JdC}^2 + 1456 \text{ JdC JpA} - \\
& 932 \text{ JdC JpB} - 660 \text{ JpA JpB} + 465 \text{ JpB}^2) + \\
& 4 \text{ JdB} (4 \text{ JdC} (180 \text{ JdC}^2 + 233 \text{ JdC JpA} + 317 \text{ JpA}^2) - 2 (728 \text{ JdC}^2 + \\
& 604 \text{ JdC JpA} + 233 \text{ JpA}^2)) \text{ JpB} + (1268 \text{ JdC} + 291 \text{ JpA}) \text{ JpB}^2 - 32 \text{ JpB}^3) - \\
& \text{ JpA} (2656 \text{ JdC}^3 + 60 \text{ JdC}^2 (31 \text{ JpA} - 44 \text{ JpB}) + \text{ JpB} (52 \text{ JpA}^2 + 561 \text{ JpA JpB} + \\
& 52 \text{ JpB}^2) + 4 \text{ JdC} (32 \text{ JpA}^2 - 291 \text{ JpA JpB} + 466 \text{ JpB}^2))) \text{ Cos}[2 \text{ k}] + \\
& (-3456 \text{ J}^2 + 14 \text{ 976 J}^2 \text{ Ja} - 16 \text{ J}^2 (1392 \text{ Ja}^2 - 540 \text{ JdB}^2 - 540 \text{ JdC}^2 - \\
& 378 \text{ JdC JpA} - 131 \text{ JpA}^2 + 54 \text{ JdB} (14 \text{ JdC} + 10 \text{ JpA} - 7 \text{ JpB}) + \\
& 540 \text{ JdC JpB} + 329 \text{ JpA JpB} - 131 \text{ JpB}^2) + \\
& \text{ Ja} (-324 \text{ Ja}^4 - 315 (-2 \text{ JdB} + \text{ JpA})^2 (-2 \text{ JdC} + \text{ JpB})^2 - \\
& 2 \text{ Ja}^2 (508 \text{ JdB}^2 + 508 \text{ JdC}^2 - 886 \text{ JdC JpA} + 123 \text{ JpA}^2 + \text{ JdB} \\
& (660 \text{ JdC} - 508 \text{ JpA} - 886 \text{ JpB}) - 508 \text{ JdC JpB} + 581 \text{ JpA JpB} + 123 \text{ JpB}^2) + \\
& 2 \text{ Ja} (2 \text{ JdC} (-308 \text{ JdB} (\text{ JdB} + \text{ JdC}) + 6 (-28 \text{ JdB} + 23 \text{ JdC}) \text{ JpA} + 155 \text{ JpA}^2) + \\
& 3 (4 \text{ JdB} (23 \text{ JdB} - 28 \text{ JdC}) + 92 (\text{ JdB} + \text{ JdC}) \text{ JpA} - 67 \text{ JpA}^2) \text{ JpB} + \\
& (310 \text{ JdB} - 201 \text{ JpA}) \text{ JpB}^2)) + \\
& 8 \text{ J}^2 (1548 \text{ Ja}^3 + 6 \text{ JdC} (-108 \text{ JdB} (\text{ JdB} + \text{ JdC}) + 54 \text{ JdC JpA} + 25 \text{ JpA}^2) + \\
& (324 \text{ JdB}^2 + 76 (\text{ JdB} + \text{ JdC}) \text{ JpA} - 113 \text{ JpA}^2) \text{ JpB} + (150 \text{ JdB} - 113 \text{ JpA}) \text{ JpB}^2 + \\
& \text{ Ja} (-1620 \text{ JdB}^2 - 1620 \text{ JdC}^2 + 178 \text{ JdC JpA} - 393 \text{ JpA}^2 + 1620 \text{ JdC JpB} + \\
& 53 \text{ JpA JpB} - 393 \text{ JpB}^2 + 2 \text{ JdB} (378 \text{ JdC} + 810 \text{ JpA} + 89 \text{ JpB}))) + \\
& 2 \text{ J}^2 (-816 \text{ Ja}^4 + 315 (-2 \text{ JdB} + \text{ JpA})^2 (-2 \text{ JdC} + \text{ JpB})^2 + 2 \text{ Ja}^2 (1588 \text{ JdB}^2 + \\
& 1588 \text{ JdC}^2 + 385 \text{ JpA}^2 + 2 \text{ JdB} (330 \text{ JdC} - 794 \text{ JpA} - 721 \text{ JpB}) + 857 \text{ JpA JpB} + \\
& 385 \text{ JpB}^2 - 2 \text{ JdC} (721 \text{ JpA} + 794 \text{ JpB})) + 4 \text{ Ja} (4 \text{ JdB}^2 (162 \text{ JdC} - 77 \text{ JpB}) + \\
& \text{ JpA} (-308 \text{ JdC}^2 + 155 \text{ JpB} (\text{ JpA} + \text{ JpB}) - 2 \text{ JdC} (113 \text{ JpA} + 84 \text{ JpB})) + 2 \text{ JdB}
\end{aligned}$$



$$\begin{aligned}
& 347 JpA^2) JpB + (112 Ja - 1330 JdB - 347 JpA) JpB^2) + \\
& 2 J2 (144 JdB (JdB - JdC) JdC (-10 Ja + 19 (JdB + JdC)) - \\
& 8 (8 Ja JdB (7 Ja + 4 JdB) + (-52 Ja^2 - 652 Ja JdB + 297 JdB^2) JdC + \\
& 18 Ja JdC^2 - 171 JdC^3) JpA + 4 (56 Ja^2 + 64 Ja JdB - 1290 Ja JdC + \\
& 545 JdB JdC + 88 JdC^2) JpA^2 + 2 (-32 Ja + 229 JdC) JpA^3 + \\
& (-8 JdB (52 Ja^2 - 18 Ja JdB + 171 JdB^2) + 32 Ja (14 Ja - 163 JdB) JdC + \\
& 8 (32 Ja + 297 JdB) JdC^2 + 4 (JdB - JdC) (324 Ja + 329 (JdB + JdC)) JpA + \\
& 2 (350 Ja - 609 JdB - 176 JdC) JpA^2 - 197 JpA^3) JpB - \\
& 2 (2 (56 Ja^2 - 1290 Ja JdB + 88 JdB^2 + 64 Ja JdC + 545 JdB JdC) + (350 Ja - \\
& 176 JdB - 609 JdC) JpA) JpB^2 + (64 Ja - 458 JdB + 197 JpA) JpB^3) + \\
& Ja^2 (4 JdB^2 (1154 JdC + 64 JpA - 613 JpB) + 4 JdC^2 (613 JpA - 64 JpB) + \\
& (JpA - JpB) (64 JpA^2 - 1299 JpA JpB + 64 JpB^2) + \\
& JdC (4462 JpA^2 - 3288 JpA JpB + 256 JpB^2) - 2 JdB \\
& (2308 JdC^2 + 128 JpA^2 + 4808 JdC (JpA - JpB) - 1644 JpA JpB + 2231 JpB^2)) + \\
& Ja (8 JdB^3 (-342 JdC + 259 JpB) - 4 JdB^2 (7 (3 JpA - 40 JpB) JpB + JdC \\
& (550 JpA + 384 JpB)) + 2 JdB (1368 JdC^3 + 4 JdC^2 (192 JpA + 275 JpB) + \\
& 98 JdC (-JpA^2 + JpB^2) + JpB (377 JpA^2 - 296 JpA JpB + 153 JpB^2)) - \\
& JpA (2072 JdC^3 + 28 JdC^2 (40 JpA - 3 JpB) + 33 JpB (-JpA^2 + JpB^2) + \\
& JdC (306 JpA^2 - 592 JpA JpB + 754 JpB^2))) \\
& \text{Sin}[2 k] - 8 i (2 JdC (2 (72 J2^2 - 72 J2 Ja + 7 Ja^2) JdB (JdB - JdC) + \\
& (4 J2 Ja (7 Ja + 4 JdB - 18 JdC) + 7 Ja^2 (-Ja + 2 JdB + JdC) + \\
& J2^2 (-28 Ja + 72 JdC)) JpA + (-70 J2^2 + 62 J2 Ja - 19 Ja^2) JpA^2) + \\
& (-2 JdB (J2^2 (-28 Ja + 72 JdB) + 7 Ja^2 (-Ja + JdB + 2 JdC) + \\
& 4 J2 Ja (7 Ja - 18 JdB + 4 JdC)) - 2 Ja (8 J2 + 7 Ja) \\
& (JdB - JdC) JpA + (70 J2^2 - 62 J2 Ja + 19 Ja^2) JpA^2) JpB + \\
& (70 J2^2 - 62 J2 Ja + 19 Ja^2) (2 JdB - JpA) JpB^2) \text{Sin}[3 k])
\end{aligned}$$

$$W12o5[k_, Ja_, J2_, JdB_, JpA_, JpB_, JdC_] := \frac{1}{1536}$$

$$\begin{aligned}
& (6 JdC (-8 JdB^2 (4 JdB + JdC) + 8 JdB (2 JdB + JdC) JpA - 2 (5 JdB + JdC) JpA^2 - 11 JpA^3) + \\
& 6 (16 JdB^3 + 14 JdB^2 JpA + 3 JpA^2 (JdC + JpA) - JdB JpA (6 JdC + JpA)) JpB - \\
& 3 (24 JdB^2 + 64 JdC^2 - 54 JdB JpA + 17 JpA^2) JpB^2 + 48 JpB^4 + \\
& 24 J2^3 (6 JdB - 8 JdC - 3 JpA + 4 JpB) + Ja^3 (-10 JdB - 72 JdC + 19 JpA + 36 JpB) - \\
& Ja^2 (124 JdB^2 + 328 JdC^2 + 31 JpA^2 + 4 JdC (33 JpA - 64 JpB) - \\
& 4 JdB (8 JdC + 35 JpA - 26 JpB) - 60 JpA JpB + 66 JpB^2) - \\
& 4 J2^2 (36 (JdB^2 - 2 JdB JdC + 2 JdC^2) + 31 JpA^2 + 92 JpA JpB + 26 JpB^2 + \\
& Ja (102 JdB - 24 JdC - 17 JpA + 12 JpB)) + \\
& Ja (-24 JdB^3 - 12 JdB^2 (4 JdC + JpA - 11 JpB) + \\
& 2 JdB (-84 JdC^2 + 114 JdC JpA + 27 JpA^2 + 272 JdC JpB - 93 JpA JpB - 71 JpB^2) + \\
& JpA (340 JdC^2 - 6 JdC JpA + 27 JpA^2 - 272 JdC JpB + 24 JpA JpB + 43 JpB^2)) + \\
& 2 J2 (3 (8 JdB (JdB^2 + 4 JdB JdC + 7 JdC^2) - 4 (11 JdB^2 + 2 JdB JdC + 7 JdC^2) JpA - \\
& 2 (JdB + 2 JdC) JpA^2 - 5 JpA^3) + \\
& 2 (12 JdB (JdB - 9 JdC) - 2 (24 JdB + 37 JdC) JpA - 9 JpA^2) JpB + \\
& (98 JdB + 19 JpA) JpB^2 + Ja^2 (-2 JdB - 120 JdC + 21 JpA + 60 JpB) + Ja (144 JdC^2 + \\
& 212 JdC JpA + 70 JpA^2 - 4 JdB (18 JdC + JpA - 52 JpB) - 20 JpA JpB + 52 JpB^2)) + \\
& (-48 JdB JdC^2 (JdB + 2 JdC) + 48 JdC^3 JpA - 4 (48 JdB^2 + 19 JdC^2) JpA^2 + 48 JpA^4 +
\end{aligned}$$

$$\begin{aligned}
& 144 J_2^3 (2 J_{dC} - J_{pB}) + 8 J_{dC} (6 J_{dB} (J_{dB} + J_{dC}) - (J_{dB} - 12 J_{dC}) J_{pA} + 19 J_{pA}^2) J_{pB} + \\
& (-28 J_{dB}^2 + (36 J_{dC} - 49 J_{pA}) J_{pA} + 20 J_{dB} (-6 J_{dC} + J_{pA})) J_{pB}^2 - \\
& 36 J_{dB} J_{pB}^3 + 2 J_a^3 (-8 J_{dB} - 10 J_{dC} + 6 J_{pA} + 5 J_{pB}) - \\
& 2 J_a^2 (160 J_{dB}^2 + 124 J_{dC}^2 + 45 J_{pA}^2 - 2 J_{dB} (12 J_{dC} + 70 J_{pA} - 35 J_{pB}) + 32 J_{dC} \\
& (4 J_{pA} - 5 J_{pB}) - 34 J_{pA} J_{pB} + 53 J_{pB}^2) + 2 J_2 (-4 J_a^2 (44 J_{dB} + J_{dC} - 20 J_{pA}) + \\
& 2 J_{dC} (108 J_{dB}^2 + 72 J_{dB} J_{dC} + 24 J_{dC}^2 - 132 J_{dB} J_{pA} + 35 J_{pA}^2) + \\
& 8 J_a (12 J_{dB}^2 - J_{dB} (21 J_{dC} + J_{pA}) + J_{pA} (50 J_{dC} + 11 J_{pA})) + (2 (J_a^2 + 106 J_a \\
& J_{dB} - 6 (9 J_{dB}^2 + 6 J_{dB} J_{dC} + 22 J_{dC}^2)) + 4 (11 J_a - 29 J_{dB} - 34 J_{dC}) J_{pA} + \\
& 29 J_{pA}^2) J_{pB} + 4 (40 J_a - 4 J_{dB} - 3 J_{dC} + 4 J_{pA}) J_{pB}^2 - 30 J_{pB}^3) + \\
& J_a (-2 J_{dC} (108 J_{dB}^2 + 24 J_{dC}^2 - 4 (69 J_{dB} + 28 J_{dC}) J_{pA} + 47 J_{pA}^2) + \\
& (4 (99 J_{dB}^2 + 62 J_{dB} J_{dC} + 66 J_{dC}^2) - 4 (79 J_{dB} + 62 J_{dC}) J_{pA} + 31 J_{pA}^2) J_{pB} + \\
& 12 (-J_{dB} + J_{dC} + 2 J_{pA}) J_{pB}^2 + 30 J_{pB}^3) - \\
& 8 J_2^2 (24 J_{dB}^2 + 36 J_{dC}^2 + 12 J_{dC} J_{pA} + 21 J_{pA}^2 + J_a (102 J_{dC} - 2 J_{pA} - 51 J_{pB}) + \\
& 86 J_{pA} J_{pB} + 31 J_{pB}^2 - 12 J_{dB} (5 J_{dC} + J_{pB})) \cos[k] - \\
& (48 J_2^3 (2 J_{dB} - 8 J_{dC} - J_{pA} + 4 J_{pB}) + 4 J_a^3 (-5 J_{dB} - 28 J_{dC} + 6 J_{pA} + 14 J_{pB}) + \\
& J_a^2 (124 J_{dB}^2 - 16 J_{dC}^2 + 8 J_{dC} J_{pA} + 75 J_{pA}^2 - \\
& 4 J_{dB} (4 J_{dC} + 45 J_{pA} - 38 J_{pB}) - 8 (4 J_{dC} + J_{pA}) J_{pB} + 40 J_{pB}^2) + 4 J_2^2 \\
& (36 J_{dB}^2 - 48 J_{dC}^2 - 24 J_{dC} J_{pA} + 31 J_{pA}^2 + 4 J_a (3 J_{dB} + 12 J_{dC} - 10 J_{pA} - 6 J_{pB}) + \\
& 80 J_{pA} J_{pB} + 32 J_{pB}^2 + 24 J_{dB} (-2 J_{dC} + J_{pB})) + \\
& 2 (24 J_{dB}^3 (-2 J_{dC} + J_{pB}) + J_{dB} J_{pA} (30 J_{dC} J_{pA} - 7 (2 J_{dC} + 3 J_{pA}) J_{pB} + 5 J_{pB}^2) + \\
& 2 J_{dB}^2 (12 J_{dC} J_{pA} + J_{pB} (-3 J_{pA} + J_{pB})) - \\
& J_{pA}^2 (-8 J_{dC}^2 + J_{pB} (-9 J_{pA} + J_{pB}) + J_{dC} (15 J_{pA} + J_{pB}))) + 2 J_2 (-24 J_{dB}^3 + \\
& 2 J_a^2 (46 J_{dB} + 56 J_{dC} - 13 J_{pA} - 28 J_{pB}) + 12 J_{dB}^2 (-4 J_{dC} + 11 J_{pA} + 2 J_{pB}) + \\
& 2 J_a (48 J_{dB} J_{dC} + 48 J_{dC}^2 - 2 J_{dB} J_{pA} - 45 J_{pA}^2 - 32 (3 J_{dB} + J_{pA}) J_{pB} - 32 J_{pB}^2) + \\
& J_{dB} (72 J_{dC}^2 + 48 J_{dC} J_{pA} + 6 J_{pA}^2 - 72 J_{dC} J_{pB} + 40 J_{pA} J_{pB} + 58 J_{pB}^2) + \\
& J_{pA} (-36 J_{dC}^2 + 15 J_{pA}^2 - 34 J_{pA} J_{pB} - 25 J_{pB}^2 + 4 J_{dC} (J_{pA} + 7 J_{pB}))) + \\
& J_a (24 J_{dB}^3 + J_{pA} (4 J_{dC}^2 + 6 J_{dC} J_{pA} - 3 J_{pA}^2 - 16 J_{dC} J_{pB} + 27 J_{pB}^2) - \\
& 4 J_{dB}^2 (12 J_{dC} + 23 (3 J_{pA} + J_{pB})) + \\
& J_{dB} (-72 J_{dC}^2 + 42 J_{pA}^2 + 62 J_{pA} J_{pB} - 78 J_{pB}^2 + 4 J_{dC} (-5 J_{pA} + 28 J_{pB}))) \cos[2k] + \\
& (-4 J_2 (2 J_a^2 (14 J_{dB} + 45 J_{dC} - 9 J_{pA}) + 15 J_{dC} (-2 J_{dB} + J_{pA})^2 + \\
& 2 J_a (12 J_{dB}^2 - 2 J_{dB} J_{pA} - 7 J_{pA}^2)) + \\
& 8 J_2^2 (12 J_{dB}^2 - 8 J_{pA}^2 + J_a (-12 J_{dB} + 90 J_{dC} + 4 J_{pA} - 45 J_{pB})) + \\
& J_a (8 J_a (J_{dB} - J_{pA}) (J_{dB} + 2 J_{pA}) + J_a^2 (56 J_{dB} + 60 J_{dC} - 32 J_{pA} - 30 J_{pB}) + \\
& 15 (-2 J_{dB} + J_{pA})^2 (2 J_{dC} - J_{pB})) + \\
& 30 J_2 (6 J_a^2 + (-2 J_{dB} + J_{pA})^2) J_{pB} + 48 J_2^3 (4 J_{dB} - 2 (5 J_{dC} + J_{pA}) + 5 J_{pB})) \\
& \cos[3k] - 15 (2 J_2 - J_a)^3 (2 J_{dB} - J_{pA}) \cos[4k] + \\
& \text{ii} (8 J_{dB} (16 J_a^3 + J_a^2 (42 J_{dB} - 2 J_{dC}) + 3 J_a J_{dC} (5 J_{dB} + 4 J_{dC}) + 6 J_{dC}^2 (J_{dB} + 6 J_{dC})) + \\
& 192 J_2^3 (2 J_{dB} - J_{pA}) - \\
& 4 (15 J_a^3 + 36 J_{dC}^3 + 2 J_a J_{dC} (67 J_{dB} + 5 J_{dC}) + 2 J_a^2 (29 J_{dB} + 6 J_{dC})) J_{pA} + \\
& 2 (21 J_a^2 + 96 J_{dB}^2 + 95 J_a J_{dC} + 34 J_{dC}^2) J_{pA}^2 - 48 J_{pA}^4 + \\
& 4 J_2 (4 J_a^2 (8 J_{dB} - 5 J_{pA}) - 3 J_{dC} (20 J_{dB}^2 + 8 J_{dB} J_{dC} - 28 J_{dB} J_{pA} + 8 J_{dC} J_{pA} + \\
& 21 J_{pA}^2) - 4 J_a (24 J_{dB}^2 + 2 J_{pA} (J_{dC} + J_{pA}) + J_{dB} (3 J_{dC} + J_{pA}))) - 2 J_2 \\
& (4 (10 J_a^2 + 53 J_a J_{dB} - 15 J_{dB}^2 - 2 J_a J_{dC} + 6 J_{dB} J_{dC}) - 4 (21 J_a + 45 J_{dB} + 14 J_{dC}) \\
& J_{pA} + 9 J_{pA}^2) J_{pB} - (28 J_a^3 - 4 J_a^2 (31 J_{dB} + 10 J_{dC} - 13 J_{pA}) +
\end{aligned}$$

$$\begin{aligned}
& 4 JdC (12 JdB (JdB + 3 JdC) + 2 (-8 JdB + 9 JdC) JpA + 43 JpA^2) + \\
& Ja (4 (71 JdB^2 + 52 JdB JdC - 72 JdC^2) - 4 (57 JdB + 31 JdC) JpA + 55 JpA^2) JpB + \\
& 8 J2 (5 Ja + 2 JdB + 13 JpA) JpB^2 - (44 Ja^2 + 4 JdB^2 + 16 (JdB - 3 JdC) JpA - \\
& 53 JpA^2 + 24 Ja (4 JdC + JpA)) JpB^2 - 12 (2 Ja - 8 JdB + 3 JpA) JpB^3 + \\
& 8 J2^2 (48 JdB^2 + 12 JdB (-JdC + JpB) + JpA (-12 JdC + 5 JpA + 6 JpB) + \\
& Ja (-24 JdB + 14 JpA + 34 JpB)) Sin[k] - i (192 J2^3 (2 JdB - JpA) - \\
& 2 JdC (-48 JdB^3 + 24 JdB^2 JpA + 30 JdB JpA^2 + (8 JdC - 15 JpA) JpA^2) + \\
& 2 (-24 JdB^3 + 6 JdB^2 JpA + (JdC - 9 JpA) JpA^2 + 7 JdB JpA (2 JdC + 3 JpA)) JpB + \\
& 2 (-2 JdB^2 - 5 JdB JpA + JpA^2) JpB^2 + Ja^3 (-40 JdB + 6 JpA + 8 JpB) + \\
& Ja^2 (-124 JdB^2 - JpA (8 JdC + 75 JpA) + 4 JdB (4 JdC + 45 JpA - 38 JpB) + \\
& 8 (2 JdC + JpA) JpB - 8 JpB^2) - 4 J2^2 (36 JdB^2 + 2 Ja (96 JdB - 65 JpA - 4 JpB) + \\
& 24 JdB (-2 JdC + JpB) + JpA (-24 JdC + 31 JpA + 80 JpB)) + \\
& 2 J2 (24 JdB^3 + 12 JdB^2 (4 JdC - 11 JpA - 2 JpB) - JpA (84 JdC^2 + 15 JpA^2 + \\
& 4 JdC (JpA - 23 JpB) - 34 JpA JpB + 5 JpB^2) + 8 Ja^2 (11 JdB - 2 (4 JpA + JpB))) + \\
& 2 JdB (84 JdC^2 - 3 JpA^2 - 20 JpA JpB + JpB^2 - 12 JdC (2 JpA + 7 JpB)) + 2 Ja \\
& (45 JpA^2 + 32 JpA JpB + 4 JpB (-2 JdC + JpB) + 2 JdB (-24 JdC + JpA + 48 JpB))) + \\
& Ja (-24 JdB^3 + 2 JdB (-84 JdC^2 + 10 JdC JpA - 21 JpA^2 + 64 JdC JpB - \\
& 31 JpA JpB + 9 JpB^2) + 4 JdB^2 (12 JdC + 23 (3 JpA + JpB)) + \\
& JpA (116 JdC^2 - 2 JdC (3 JpA + 52 JpB) + 3 (JpA^2 + JpB^2))) Sin[2 k] - \\
& i (96 J2^3 (2 JdB - JpA) + 32 J2^2 (3 JdB (-Ja + JdB) + Ja JpA - 2 JpA^2) + \\
& 4 J2 (-15 JdC (-2 JdB + JpA))^2 + Ja^2 (-28 JdB + 18 JpA) + \\
& Ja (-24 JdB^2 + 4 JdB JpA + 14 JpA^2)) + Ja (8 Ja^2 (7 JdB - 4 JpA) + \\
& 8 Ja (JdB - JpA) (JdB + 2 JpA) + 15 (-2 JdB + JpA)^2 (2 JdC - JpB)) + \\
& 30 J2 (-2 JdB + JpA)^2 JpB Sin[3 k] + 15 i (2 J2 - Ja)^3 (2 JdB - JpA) Sin[4 k]
\end{aligned}$$

(\* We report first 7 orders of the ground-state energy per dimer. Normalization : Jd=1. \*)

(\* ZEROth ORDER \*)

gs0[Ja\_, J2\_, JdB\_, JpA\_, JpB\_, JdC\_] := 1;

(\* FIRST ORDER \*)

gs1[Ja\_, J2\_, JdB\_, JpA\_, JpB\_, JdC\_] := 0;

(\* SECOND ORDER \*)

gs2[Ja\_, J2\_, JdB\_, JpA\_, JpB\_, JdC\_] :=  
(-3 \* (4 \* (JdC - JpB) \* JdC + JpA^2 + JpB^2 + 4 \* (JdB - JpA) \* JdB +  
2 \* Ja^2 + 8 \* (J2 - Ja) \* J2)) / 64;

(\* THIRD ORDER \*)

gs3[Ja\_, J2\_, JdB\_, JpA\_, JpB\_, JdC\_] :=  
(-3 \* (2 \* (4 \* JdC^2 - 2 \* JdC \* JpB - JpB^2) \* JdC +  
(JpA^2 - JpA \* JpB + JpB^2) \* (JpA + JpB) + 2 \* (4 \* JdB^2 - 2 \* JdB \* JpA - JpA^2) \*  
JdB + 2 \* (3 \* (2 \* JdB - JpA) \* (2 \* JdC - JpB) + Ja^2) \* Ja -  
4 \* (3 \* (2 \* JdB - JpA) \* (2 \* JdC - JpB) + Ja^2 - 2 \* (2 \* J2 - Ja) \* J2) \* J2)) / 256;

(\* FOURTH ORDER \*)

```

gs4[Ja_, J2_, JdB_, JpA_, JpB_, JdC_] :=
(16 * ((12 * (3 * JpA - 2 * JpB + 4 * JdC - 3 * JdB) * JdB - (12 * (2 * JpA - 3 * JpB + 3 * JdC) *
      JdC + 13 * JpA^2 - 8 * JpA * JpB + 13 * JpB^2) + 49 * Ja^2 +
      6 * (J2 - 10 * Ja) * J2) * J2 + (4 * (JpA - 9 * JpB + 9 * JdC) * JdC +
      13 * (JpA^2 + JpB^2) - 4 * (9 * JpA - JpB - 9 * JdB) * JdB - 7 * Ja^2) * Ja -
      2 * (2 * ((JpA + 4 * JpB) * JpB - 12 * JdC^2 - 6 * (2 * JdC - JpB) * JdB) * JdB -
      (5 * (JpA + JpB) * JpB - 12 * JdC^2 - 2 * (4 * JpA + JpB) * JdC) * JpA)) * J2 +
      2 * (8 * (2 * (2 * (JpA + JpB - 6 * JdC) * JdC - (2 * JpA - 3 * JpB) * JpB -
      4 * (3 * JdC - 2 * JpB) * JdB) * JdB -
      (3 * (JpA + JpB) * JpB - 16 * JdC^2 - 2 * (3 * JpA - 2 * JpB) * JdC) * JpA) -
      (13 * Ja^2 + 104 * JdB^2 + 128 * JdB * JdC - 104 * JdB * JpA -
      48 * JdB * JpB + 104 * JdC^2 - 48 * JdC * JpA - 104 * JdC * JpB +
      34 * JpA^2 + 24 * JpA * JpB + 34 * JpB^2) * Ja) * Ja -
      (8 * (6 * (JdC + 6 * JpB) * JdC^2 - (2 * JpA^2 - 9 * JpB^2) * JpB -
      (2 * JpA^2 + 39 * JpB^2) * JdC) * JdC +
      3 * JpA^4 + 20 * JpA^2 * JpB^2 + 3 * JpB^4 - 8 *
      ((24 * (JdC - JpB) * JdC + 39 * JpA^2 + 2 * JpB^2 - 6 * (JdB + 6 * JpA) * JdB) * JdB -
      (8 * (3 * JdC - 2 * JpB) * JdC + 9 * JpA^2 - 2 * JpB^2) * JpA) * JdB)) / 4096;

```

(\* FIFTH ORDER \*)

```

gs5[Ja_, J2_, JdB_, JpA_, JpB_, JdC_] :=
(2 * (2 * (2 * (170 * JpA + 29 * JpB - 302 * JdC - 212 * JdB) * JdB +
      4 * (131 * (JpA + JpB) - 151 * JdC) * JdC + 74 * JpA^2 - 38 * JpA * JpB -
      115 * JpB^2) * JdB + 4 * (29 * JpA + 170 * JpB - 212 * JdC) * JdC^2 -
      11 * (14 * JpA^2 - 13 * JpA * JpB + 14 * JpB^2) * (JpA + JpB) -
      2 * (115 * JpA^2 + 38 * JpA * JpB - 74 * JpB^2) * JdC -
      (89 * Ja^2 + 520 * JdB^2 + 1472 * JdB * JdC - 520 * JdB * JpA -
      776 * JdB * JpB + 520 * JdC^2 - 776 * JdC * JpA - 520 * JdC * JpB +
      154 * JpA^2 + 400 * JpA * JpB + 154 * JpB^2) * Ja) * Ja^2 -
      (8 * (2 * (90 * (JpA + JpB - 2 * JdC) * JdC - (82 * JpA - 25 * JpB) * JpB) * JdC -
      (117 * JpA^3 - 9 * JpA * JpB^2 + 17 * JpB^3)) * JdB^2 -
      (144 * (10 * JdB - 31 * JpA) * JdB^4 + 1440 * JdC^5 - 4464 * JdC^4 * JpB +
      272 * JdC^3 * JpA^2 + 1872 * JdC^3 * JpB^2 + 136 * JdC^2 * JpA^3 -
      72 * JdC^2 * JpA^2 * JpB + 936 * JdC^2 * JpB^3 + 88 * JdC * JpA^3 * JpB +
      204 * JdC * JpA^2 * JpB^2 - 558 * JdC * JpB^4 + 45 * JpA^5 -
      134 * JpA^3 * JpB^2 - 134 * JpA^2 * JpB^3 + 45 * JpB^5 +
      16 * (180 * (JdC - JpB) * JdC + 117 * JpA^2 + 17 * JpB^2) * JdB^3) -
      2 * (8 * ((JpA + JpB) * JpB - 180 * JdC^2 - (25 * JpA - 82 * JpB) * JdC) * JdC -
      (279 * JpA^3 - 102 * JpA * JpB^2 - 44 * JpB^3)) * JdB * JpA) +
      8 * ((4 * (7 * (JpA + 21 * JpB) - 46 * JdC) * JdC^2 + (JpA^2 - 22 * JpA * JpB + JpB^2) *
      JpB - 2 * (20 * JpA^2 - 6 * JpA * JpB + 129 * JpB^2) * JdC) * JpA +
      4 * (180 * JdB * JdC - 46 * JdB * JpB - 72 * JdC^2 - 388 * JdC * JpA + 44 * JdC * JpB +
      147 * JpA * JpB + 7 * JpB^2) * JdB^2 + 2 * (8 * (11 * JpA - 97 * JpB + 45 * JdC) *
      JdC^2 - (129 * JpA^2 - 6 * JpA * JpB + 20 * JpB^2) * JpB +
      2 * (173 * JpA^2 - 30 * JpA * JpB + 173 * JpB^2) * JdC) * JdB) * Ja +

```

$$\begin{aligned}
& 4 * ((2 * (4 * (65 * JpA - 18 * JpB + 36 * JdC) * JdC^2 + (130 * JpA^2 - 121 * JpA * JpB + \\
& \quad 130 * JpB^2) * (JpA + JpB) + 2 * (131 * JpA^2 - 78 * JpA * JpB - \\
& \quad 114 * JpB^2) * JdC - 2 * (2 * (18 * JpA - 65 * JpB - 126 * JdC - 36 * JdB) * \\
& \quad \quad JdB + 4 * (83 * (JpA + JpB) - 63 * JdC) * JdC + 114 * JpA^2 + 78 * JpA * \\
& \quad \quad JpB - 131 * JpB^2) * JdB) - (133 * Ja^2 - 456 * JdB^2 - 256 * JdB * \\
& \quad \quad JdC + 456 * JdB * JpA + 336 * JdB * JpB - 456 * JdC^2 + 336 * JdC * JpA + \\
& \quad \quad 456 * JdC * JpB - 74 * JpA^2 - 136 * JpA * JpB - 74 * JpB^2) * Ja) * Ja + \\
& 8 * ((6 * (6 * (2 * JpA + 23 * JpB - 10 * JdC) * JdC - (61 * JpA^2 + 10 * JpA * JpB + 61 * \\
& \quad JpB^2)) * JdC + (149 * JpA^2 + 10 * JpA * JpB + 17 * JpB^2) * JpB + \\
& \quad 18 * (2 * (23 * JpA + 2 * JpB) * JdC - (22 * JpA + 3 * JpB) * JpB - \\
& \quad 10 * (2 * JdC - JpB) * JdB) * JdB) * JdB - (2 * (9 * (3 * JpA + 22 * JpB - \\
& \quad 10 * JdC) * JdC^2 - (2 * JpA^2 + 7 * JpA * JpB + 2 * JpB^2) * JpB) - \\
& \quad (17 * JpA^2 + 10 * JpA * JpB + 149 * JpB^2) * JdC) * JpA) - \\
& 2 * (2 * (12 * (17 * JpA + 3 * JpB - 3 * JdC) * JdC - (85 * JpA^2 + 184 * JpA * JpB + \\
& \quad 85 * JpB^2) + 12 * (3 * JpA + 17 * JpB - 48 * JdC - 3 * JdB) * JdB - \\
& \quad 127 * Ja^2) * Ja + 36 * (11 * JpA - 2 * JpB + 4 * JdC) * JdC^2 + \\
& \quad 5 * (26 * JpA^2 - 27 * JpA * JpB + 26 * JpB^2) * (JpA + JpB) + \\
& \quad 2 * (151 * JpA^2 - 122 * JpA * JpB - 114 * JpB^2) * JdC - \\
& \quad 2 * (18 * (2 * JpA - 11 * JpB - 6 * JdC - 4 * JdB) * JdB + 36 * (7 * (JpA + JpB) - \\
& \quad 3 * JdC) * JdC + 114 * JpA^2 + 122 * JpA * JpB - 151 * JpB^2) * JdB + \\
& \quad 4 * (36 * (JdC - JpB) * JdC + 53 * JpA^2 + 60 * JpA * JpB + 53 * JpB^2 + \\
& \quad 36 * (JdB - JpA) * JdB - 191 * Ja^2 - \\
& \quad 9 * (30 * J2 - 61 * Ja) * J2) * J2) * J2) / 49152;
\end{aligned}$$

(\* SIXTH ORDER \*)

gs6[Ja\_, J2\_, JdB\_, JpA\_, JpB\_, JdC\_] :=

$$\begin{aligned}
& (- (2 * ((2 * (2 * (2 * (15638 * JpA + 2227 * JpB - 718 * JdC) * JdC - \\
& \quad (1981 * JpA^2 + 31392 * JpA * JpB + 1981 * JpB^2)) * JdC + \\
& \quad 9204 * JpA^3 - 69 * JpA^2 * JpB + 11258 * JpA * JpB^2 + 729 * JpB^3 + \\
& \quad 2 * (2 * (7924 * JpA + 41 * JpB - 718 * JdC - 2050 * JdB) * JdB + \\
& \quad 2 * (2227 * JpA + 15638 * JpB - 16854 * JdC) * JdC - \\
& \quad (14918 * JpA^2 + 641 * JpA * JpB + 5191 * JpB^2)) * JdB) * JdB + \\
& \quad 2 * (2 * (2 * (41 * JpA + 7924 * JpB - 2050 * JdC) * JdC - (5191 * JpA^2 + \\
& \quad 641 * JpA * JpB + 14918 * JpB^2)) * JdC + 729 * JpA^3 + \\
& \quad 11258 * JpA^2 * JpB - 69 * JpA * JpB^2 + 9204 * JpB^3) * JdC - \\
& \quad (833 * JpA^4 - 613 * JpA^3 * JpB + 2799 * JpA^2 * JpB^2 - 613 * JpA * \\
& \quad JpB^3 + 833 * JpB^4) - ((4 * (3859 * JpA + 2657 * JpB - 2891 * JdC) * \\
& \quad JdC - (2731 * JpA^2 + 7864 * JpA * JpB + 2731 * JpB^2) + \\
& \quad 4 * (2657 * JpA + 3859 * JpB - 6600 * JdC - 2891 * JdB) * JdB - \\
& \quad 1389 * Ja^2) * Ja + 2 * (2 * (3493 * JpA + 3070 * JpB - 3292 * JdC) * \\
& \quad JdC + 1211 * JpA^2 - 3982 * JpA * JpB - 74 * JpB^2) * JdC - \\
& \quad (1302 * JpA^2 - 355 * JpA * JpB + 1302 * JpB^2) * (JpA + JpB) + \\
& \quad 2 * (2 * (3070 * JpA + 3493 * JpB - 7986 * JdC - 3292 * JdB) * JdB + \\
& \quad 4 * (2059 * (JpA + JpB) - 3993 * JdC) * JdC - \\
& \quad (74 * JpA^2 + 3982 * JpA * JpB - 1211 * JpB^2)) * JdB) * Ja) * Ja +
\end{aligned}$$

$$\begin{aligned}
& 2 * (2 * (2 * (4 * (2 * (29 * (82 * JpA + JpB) - 540 * JdC) * JdC - \\
& \quad (2262 * JpA - 211 * JpB) * JpB - (3726 * JdC - 1471 * JpB) * JdB) * \\
& \quad JdB + 2 * (2 * (2407 * (JpA + JpB) - 1080 * JdC) * JdC - \\
& \quad (1162 * JpA^2 + 1257 * JpA * JpB + 2610 * JpB^2)) * JdC + \\
& \quad (2114 * JpA^2 - 1276 * JpA * JpB + 491 * JpB^2) * JpB) * JdB + \\
& 4 * (2 * (2 * (29 * (JpA + 82 * JpB) - 1863 * JdC) * JdC^2 - \\
& \quad (687 * JpA^2 - 1163 * JpA * JpB + 687 * JpB^2) * (JpA + JpB)) - \\
& \quad (2610 * JpA^2 + 1257 * JpA * JpB + 1162 * JpB^2) * JdC) * JdC + \\
& (1156 * JpA^3 + 382 * JpA^2 * JpB - 573 * JpA * JpB^2 + 841 * JpB^3) * \\
& JpB) * JdB + (16 * (211 * JpA - 2262 * JpB + 1471 * JdC) * JdC^3 - \\
& (41 * JpA^2 - 633 * JpA * JpB + 41 * JpB^2) * (JpA + JpB) * JpB + \\
& 4 * (491 * JpA^2 - 1276 * JpA * JpB + 2114 * JpB^2) * JdC^2 + \\
& 2 * (841 * JpA^3 - 573 * JpA^2 * JpB + 382 * JpA * JpB^2 + \\
& \quad 1156 * JpB^3) * JdC) * JpA) * Ja - \\
(4 * ((16 * ((378 * JdC^2 - 540 * JdC * JpA + 756 * JdC * JpB - 845 * JpA^2 + \\
& \quad 182 * JpA * JpB - 845 * JpB^2) * JdC + \\
& \quad (352 * JpA^2 + 97 * JpA * JpB + 141 * JpB^2) * JpB) * JdC - \\
& (4401 * JpA^4 - 3236 * JpA^2 * JpB^2 + 264 * JpA * JpB^3 - \\
& \quad 106 * JpB^4) + 4 * (216 * (7 * JdC - 8 * JpB) * JdC - \\
& \quad (4401 * JpA^2 - 310 * JpB^2) + 108 * (19 * JdB - 17 * JpA) * JdB) * \\
& JdB^2 + 8 * (4 * (54 * (7 * JpA - 5 * JpB + 10 * JdC) * JdC - \\
& \quad (206 * JpA + 85 * JpB) * JpB) * JdC + 2403 * JpA^3 - \\
& \quad 298 * JpA * JpB^2 + 106 * JpB^3) * JdB) * JdB - \\
& (8 * (4 * (85 * JpA + 206 * JpB + 216 * JdC) * JdC^2 + 7 * (2 * JpA^2 + \\
& \quad 19 * JpA * JpB + 2 * JpB^2) * JpB - 2 * (141 * JpA^2 + \\
& \quad 97 * JpA * JpB + 352 * JpB^2) * JdC) * JdC + 459 * JpA^4 + 836 * \\
& \quad JpA^2 * JpB^2 - 708 * JpA * JpB^3 - 160 * JpB^4) * JpA) * JdB + \\
& 4 * ((4 * ((108 * (19 * JdC - 17 * JpB) * JdC + 310 * JpA^2 - 4401 * JpB^2) * JdC + \\
& \quad 2 * (106 * JpA^3 - 298 * JpA^2 * JpB + 2403 * JpB^3)) * JdC + 106 * \\
& \quad JpA^4 - 264 * JpA^3 * JpB + 3236 * JpA^2 * JpB^2 - 4401 * JpB^4) * JdC + \\
& (160 * JpA^4 + 708 * JpA^3 * JpB - 836 * JpA^2 * JpB^2 - 459 * JpB^4) * JpB) * \\
& JdC + 513 * JpA^6 - 938 * JpA^4 * JpB^2 - 1928 * JpA^3 * \\
& \quad JpB^3 - 938 * JpA^2 * \\
& \quad JpB^4 + 513 * JpB^6) - \\
& 4 * ((2 * (2 * (4 * (7668 * JpA - 19 * JpB + 594 * JdC - 3618 * JdB) * JdB^2 + \\
& \quad 2 * (1188 * JdC^2 + 36338 * JdC * JpA - 1742 * JdC * JpB - \\
& \quad 57 * JpA^2 - 38388 * JpA * JpB - 57 * JpB^2) * JdC + \\
& \quad 6420 * JpA^3 - 677 * JpA^2 * JpB + 16307 * JpA * JpB^2 + \\
& \quad 1111 * JpB^3 - 2 * (2 * (871 * JpA - 18169 * JpB + 18306 * JdC) * JdC + \\
& \quad 11574 * JpA^2 - 793 * JpA * JpB + 7110 * JpB^2) * JdB) * JdB - \\
& (2 * (2 * (2 * (19 * JpA - 7668 * JpB + 3618 * JdC) * JdC + \\
& \quad 7110 * JpA^2 - 793 * JpA * JpB + 11574 * JpB^2) * JdC - \\
& (1111 * JpA^3 + 16307 * JpA^2 * JpB - 677 * JpA * JpB^2 + \\
& \quad 6420 * JpB^3)) * JdC + 353 * JpA^4 + 17 * JpA^3 * JpB + \\
& \quad 6399 * JpA^2 * JpB^2 + 17 * JpA * JpB^3 + 353 * JpB^4)) -
\end{aligned}$$

$$\begin{aligned}
& (2 * (2 * (1902 * JpA + 719 * JpB - 3410 * JdC - 2172 * JdB) * JdB + \\
& \quad 4 * (551 * (JpA + JpB) - 1705 * JdC) * JdC - \\
& \quad (234 * JpA^2 + 2206 * JpA * JpB - 2595 * JpB^2)) * JdB + \\
& \quad 4 * (719 * JpA + 1902 * JpB - 2172 * JdC) * JdC^2 + \\
& \quad (74 * JpA^2 - 147 * JpA * JpB + 74 * JpB^2) * (JpA + JpB) + \\
& \quad 2 * (2595 * JpA^2 - 2206 * JpA * JpB - 234 * JpB^2) * JdC - \\
& \quad 2 * (2 * ((3408 * JdC - 1748 * JpA - 3743 * JpB + 2540 * JdB) * JdB + \\
& \quad (2540 * JdC - 3743 * JpA - 1748 * JpB) * JdC - (119 * JpA^2 - \\
& \quad 1611 * JpA * JpB + 119 * JpB^2))) - 427 * Ja^2) * Ja) * \\
Ja + 2 * (2 * (2 * (2 * (216 * (23 * (JpA + JpB) - 14 * JdC) * JdC + \\
\quad 90 * JpA^2 + 133 * JpA * JpB - 1756 * JpB^2) * JdC - \\
\quad (198 * JpA^2 + 2855 * JpA * JpB + 68 * JpB^2) * JpB - \\
\quad 4 * (3618 * JdB * JdC - 1863 * JdB * JpB + 1512 * JdC^2 - 4428 * JdC * \\
\quad JpA - 216 * JdC * JpB + 2178 * JpA * JpB - 292 * JpB^2) * JdB) * \\
JdB - (4 * ((108 * (67 * JdC - 4 * JpA - 82 * JpB) * JdC + \\
\quad 1756 * JpA^2 - 133 * JpA * JpB - 90 * JpB^2) * JdC + \\
\quad (2010 * JpA^2 - 1489 * JpA * JpB + 2010 * JpB^2) * \\
\quad (JpA + JpB))) * JdC - (3244 * JpA^3 + 2386 * JpA^2 * JpB + \\
\quad 513 * JpA * JpB^2 + 1135 * JpB^3) * JpB)) * JdB + \\
(4 * (4 * (1863 * JdC + 292 * JpA - 2178 * JpB) * JdC - (68 * JpA^2 + \\
\quad 2855 * JpA * JpB + 198 * JpB^2))) * JdC^2 - \\
(377 * JpA^2 - 538 * JpA * JpB + 377 * JpB^2) * (JpA + JpB) * \\
JpB + 2 * (1135 * JpA^3 + 513 * JpA^2 * JpB + \\
\quad 2386 * JpA * JpB^2 + 3244 * JpB^3) * JdC) * JpA) - \\
2 * (2 * (2 * (54 * (712 * JpA - 127 * JpB + 78 * JdC) * JdC + 1335 * JpA^2 - \\
\quad 42688 * JpA * JpB + 1335 * JpB^2) * JdC + 5700 * JpA^3 - \\
\quad 1561 * JpA^2 * JpB + 18872 * JpA * JpB^2 + 1385 * JpB^3 + \\
\quad 6 * (18 * (268 * JpA - 17 * JpB + 78 * JdC - 126 * JdB) * JdB - \\
\quad (18 * (127 * JpA - 712 * JpB + 642 * JdC) * JdC + 3594 * JpA^2 - \\
\quad 837 * JpA * JpB + 2711 * JpB^2))) * JdB) * JdB - \\
(2 * (6 * (18 * (17 * JpA - 268 * JpB + 126 * JdC) * JdC + 2711 * JpA^2 - \\
\quad 837 * JpA * JpB + 3594 * JpB^2) * JdC - (1385 * JpA^3 + \\
\quad 18872 * JpA^2 * JpB - 1561 * JpA * JpB^2 + 5700 * JpB^3))) * \\
JdC + 101 * JpA^4 + 275 * JpA^3 * JpB + 7779 * JpA^2 * \\
JpB^2 + 275 * JpA * JpB^3 + 101 * JpB^4) + \\
(2 * (18 * (215 * JpA - 42 * JpB + 84 * JdC) * JdC - \\
\quad (831 * JpA^2 - 2794 * JpA * JpB - 1902 * JpB^2))) * JdC - \\
(3070 * JpA^2 + 1459 * JpA * JpB + 3070 * JpB^2) * (JpA + JpB) - \\
2 * (18 * (42 * JpA - 215 * JpB + 606 * JdC - 84 * JdB) * JdB - \\
\quad (4 * (1097 * (JpA + JpB) - 2727 * JdC) * JdC + \\
\quad 1902 * JpA^2 + 2794 * JpA * JpB - 831 * JpB^2))) * JdB + \\
(1967 * Ja^2 - 4040 * JdB^2 + 12976 * JdB * JdC + 8216 * JdB * JpA - \\
\quad 13612 * JdB * JpB - 4040 * JdC^2 - 13612 * JdC * JpA + 8216 * JdC * \\
\quad JpB - 6214 * JpA^2 + 3616 * JpA * JpB - 6214 * JpB^2) * Ja) * \\
Ja - 2 * (2 * (108 * (82 * JpA - 13 * JpB + 7 * JdC) * JdC -
\end{aligned}$$

$$\begin{aligned}
& (159 * JpA^2 + 5216 * JpA * JpB + 159 * JpB^2) - \\
& 108 * (13 * JpA - 82 * JpB + 156 * JdC - 7 * JdB) * JdB - \\
& 9435 * Ja^2 + 108 * (53 * J2 - 25 * Ja) * J2) * J2 - \\
& (2 * (54 * (14 * JpA - 11 * JpB + 58 * JdC - 28 * JdB) * JdB - \\
& (108 * (9 * (JpA + JpB) - 29 * JdC) * JdC + \\
& 1086 * JpA^2 + 1678 * JpA * JpB - 411 * JpB^2)) * \\
& JdB - (2 * (54 * (11 * JpA - 14 * JpB + 28 * JdC) * JdC - \\
& (411 * JpA^2 - 1678 * JpA * JpB - 1086 * JpB^2)) * JdC - \\
& (1646 * JpA^2 + 253 * JpA * JpB + 1646 * JpB^2) * (JpA + JpB)) - \\
& 4 * ((9936 * JdC + 2052 * JpA - 5377 * JpB - 1404 * JdB) * JdB - \\
& ((1404 * JdC + 5377 * JpA - 2052 * JpB) * JdC + \\
& 851 * JpA^2 - 2385 * JpA * JpB + 851 * JpB^2) + \\
& 3391 * Ja^2) * Ja)) * J2) * J2) * J2) / 1179648;
\end{aligned}$$

(\* SEVENTH ORDER \*)

gs7[Ja\_, J2\_, JdB\_, JpA\_, JpB\_, JdC\_] :=

$$\begin{aligned}
& (4 * (((4 * ((4 * (2150545 * JpA + 306707 * JpB - 459455 * JdC) * JdC - (571128 * JpA^2 + \\
& 4170722 * JpA * JpB + 53139 * JpB^2) - 4 * (1333894 * JdC - \\
& 167736 * JpA - 639131 * JpB + 46020 * JdB) * JdB) * JdB + \\
& 2 * (2 * (306707 * JpA + 2150545 * JpB - 1333894 * JdC) * JdC - \\
& (2217297 * JpA^2 + 396442 * JpA * JpB + 2217297 * JpB^2)) * \\
& JdC + 157272 * JpA^3 + 2195749 * JpA^2 * JpB - \\
& 945 * JpA * JpB^2 + 650843 * JpB^3) * JdB - \\
& (4 * ((4 * (46020 * JdC - 639131 * JpA - 167736 * JpB) * JdC + \\
& 53139 * JpA^2 + 4170722 * JpA * JpB + 571128 * JpB^2) * \\
& JdC - (650843 * JpA^3 - 945 * JpA^2 * JpB + \\
& 2195749 * JpA * JpB^2 + 157272 * JpB^3)) * JdC + \\
& 74916 * JpA^4 + 1445886 * JpA^3 * JpB - 54449 * JpA^2 * \\
& JpB^2 + 1445886 * JpA * JpB^3 + 74916 * JpB^4) - \\
& (4 * (4 * (73178 * JpA + 26517 * JpB - 45954 * JdC) * JdC^2 + (17411 * \\
& JpA^2 - 42107 * JpA * JpB + 17411 * JpB^2) * (JpA + JpB) + \\
& 2 * (58794 * JpA^2 - 72050 * JpA * JpB - 8935 * JpB^2) * JdC + \\
& 2 * (2 * (26517 * JpA + 73178 * JpB - 115180 * JdC - 45954 * JdB) * \\
& JdB + 8 * (10184 * (JpA + JpB) - 28795 * JdC) * JdC - \\
& (8935 * JpA^2 + 72050 * JpA * JpB - 58794 * JpB^2)) * JdB) + \\
& (94795 * Ja^2 - 1286872 * JdB^2 - 1137496 * JdB * JdC + \\
& 1119544 * JdB * JpA + 681628 * JdB * JpB - 1286872 * JdC^2 + \\
& 681628 * JdC * JpA + 1119544 * JdC * JpB - 325958 * JpA^2 - \\
& 178366 * JpA * JpB - 325958 * JpB^2) * Ja) * Ja) * Ja + \\
& 2 * (2 * (4 * (4 * (479761 * JpA + 91384 * JpB - 35154 * JdC) * JdC^2 + \\
& (120096 * JpA^2 - 440675 * JpA * JpB + 120096 * JpB^2) * \\
& (JpA + JpB) + (392041 * JpA^2 - 1299758 * JpA * JpB - 350100 * \\
& JpB^2) * JdC) * JdC + 436080 * JpA^4 - 26544 * JpA^3 * JpB + \\
& 159569 * JpA^2 * JpB^2 + 749274 * JpA * JpB^3 - 11178 * JpB^4 + \\
& 2 * (2 * (4 * (170424 * JpA - 24245 * JpB - 35154 * JdC - 110160 * JdB) *
\end{aligned}$$

$$\begin{aligned}
& \text{JdB} + 4 * (91\,384 * \text{JpA} + 479\,761 * \text{JpB} - 452\,385 * \text{JdC}) * \text{JdC} - \\
& (192\,672 * \text{JpA}^2 - 133\,216 * \text{JpA} * \text{JpB} + 492\,417 * \text{JpB}^2) * \\
& \text{JdB} + 2 * (90 * (12\,101 * (\text{JpA} + \text{JpB}) - 20\,106 * \text{JdC}) * \text{JdC} - \\
& (350\,100 * \text{JpA}^2 + 1\,299\,758 * \text{JpA} * \text{JpB} - 392\,041 * \text{JpB}^2)) * \\
& \text{JdC} - (372\,384 * \text{JpA}^3 + 64\,308 * \text{JpA}^2 * \text{JpB} - \\
& 755\,437 * \text{JpA} * \text{JpB}^2 + 363\,625 * \text{JpB}^3) * \text{JdB} * \text{JdB} - \\
& (2 * (2 * (2 * (4 * (24\,245 * \text{JpA} - 170\,424 * \text{JpB} + 110\,160 * \text{JdC}) * \text{JdC} + \\
& 492\,417 * \text{JpA}^2 - 133\,216 * \text{JpA} * \text{JpB} + 192\,672 * \text{JpB}^2) * \\
& \text{JdC} + 363\,625 * \text{JpA}^3 - 755\,437 * \text{JpA}^2 * \text{JpB} + \\
& 64\,308 * \text{JpA} * \text{JpB}^2 + 372\,384 * \text{JpB}^3) * \text{JdC} + \\
& 11\,178 * \text{JpA}^4 - 749\,274 * \text{JpA}^3 * \text{JpB} - 159\,569 * \text{JpA}^2 * \\
& \text{JpB}^2 + 26\,544 * \text{JpA} * \text{JpB}^3 - 436\,080 * \text{JpB}^4) * \text{JdC} + \\
& (89\,168 * \text{JpA}^4 - 96\,094 * \text{JpA}^3 * \text{JpB} + 365\,275 * \text{JpA}^2 * \text{JpB}^2 - \\
& 96\,094 * \text{JpA} * \text{JpB}^3 + 89\,168 * \text{JpB}^4) * (\text{JpA} + \text{JpB}))) * \text{Ja} - \\
& (4 * ((4 * ((324 * (1348 * \text{JpA} + 227 * \text{JpB} + 779 * \text{JdC}) * \text{JdC} - (174\,312 * \text{JpA} + \\
& 127\,909 * \text{JpB}) * \text{JpB} + 1296 * (242 * \text{JdC} - 139 * \text{JpB}) * \text{JdB}) * \\
& \text{JdB} - 2 * (4 * (81 * (436 * \text{JdC} + 259 * \text{JpA} - 1134 * \text{JpB}) * \text{JdC} + \\
& 145\,422 * \text{JpA}^2 + 27\,802 * \text{JpA} * \text{JpB} + 38\,225 * \text{JpB}^2) * \text{JdC} - \\
& (252\,324 * \text{JpA}^2 + 89\,519 * \text{JpA} * \text{JpB} + 34\,78 * \text{JpB}^2) * \text{JpB})) * \\
& \text{JdB} + 8 * ((162 * (779 * \text{JdC} + 2268 * \text{JpA} - 518 * \text{JpB}) * \text{JdC} - \\
& (81\,971 * \text{JpA}^2 + 738\,580 * \text{JpA} * \text{JpB} + 81\,971 * \text{JpB}^2)) * \text{JdC} + \\
& 259\,092 * \text{JpA}^3 + 74\,995 * \text{JpA}^2 * \text{JpB} + 239\,482 * \text{JpA} * \text{JpB}^2 + \\
& 61\,361 * \text{JpB}^3) * \text{JdC} - (801\,360 * \text{JpA}^3 + 124\,254 * \text{JpA}^2 * \text{JpB} - \\
& 116\,072 * \text{JpA} * \text{JpB}^2 + 41\,245 * \text{JpB}^3) * \text{JpB}) * \text{JdB} + \\
& 8 * ((2 * (78\,408 * \text{JdC}^2 + 18\,387 * \text{JdC} * \text{JpA} + 109\,188 * \text{JdC} * \text{JpB} - \\
& 76\,450 * \text{JpA}^2 - 55\,604 * \text{JpA} * \text{JpB} - 290\,844 * \text{JpB}^2) * \\
& \text{JdC} + 61\,361 * \text{JpA}^3 + 239\,482 * \text{JpA}^2 * \text{JpB} + \\
& 74\,995 * \text{JpA} * \text{JpB}^2 + 259\,092 * \text{JpB}^3) * \text{JdC} - \\
& (11\,019 * \text{JpA}^4 + 10\,684 * \text{JpA}^3 * \text{JpB} + 27\,825 * \text{JpA}^2 * \text{JpB}^2 + \\
& 10\,684 * \text{JpA} * \text{JpB}^3 + 11\,019 * \text{JpB}^4) * \text{JdC} + \\
& (14\,372 * \text{JpA}^4 - 61\,922 * \text{JpA}^3 * \text{JpB} - 149\,884 * \text{JpA}^2 * \text{JpB}^2 - \\
& 10\,321 * \text{JpA} * \text{JpB}^3 - 34\,540 * \text{JpB}^4) * \text{JpB}) * \text{JdB} - \\
& (4 * (4 * ((127\,909 * \text{JpA} + 174\,312 * \text{JpB} + 180\,144 * \text{JdC}) * \text{JdC} - \\
& 2 * (34\,78 * \text{JpA}^2 + 89\,519 * \text{JpA} * \text{JpB} + 252\,324 * \text{JpB}^2)) * \\
& \text{JdC} + 41\,245 * \text{JpA}^3 - 116\,072 * \text{JpA}^2 * \text{JpB} + \\
& 124\,254 * \text{JpA} * \text{JpB}^2 + 801\,360 * \text{JpB}^3) * \text{JdC}^2 - \\
& (15\,160 * \text{JpA}^4 - 9\,733 * \text{JpA}^3 * \text{JpB} + 70\,872 * \text{JpA}^2 * \text{JpB}^2 - \\
& 9\,733 * \text{JpA} * \text{JpB}^3 + 15\,160 * \text{JpB}^4) * \text{JpB} + \\
& 4 * (34\,540 * \text{JpA}^4 + 10\,321 * \text{JpA}^3 * \text{JpB} + 149\,884 * \text{JpA}^2 * \text{JpB}^2 + \\
& 61\,922 * \text{JpA} * \text{JpB}^3 - 14\,372 * \text{JpB}^4) * \text{JdC}) * \text{JpA}) - \\
& 2 * ((4 * ((4 * (1\,778\,067 * \text{JpA} - 456\,149 * \text{JpB} + 342\,387 * \text{JdC}) * \text{JdC} + \\
& 213\,624 * \text{JpA}^2 - 3\,520\,962 * \text{JpA} * \text{JpB} + 616\,315 * \text{JpB}^2 - \\
& 36 * (71\,28 * \text{JpA} - 67\,043 * \text{JpB} + 135\,882 * \text{JdC} - 4644 * \text{JdB}) * \text{JdB}) * \\
& \text{JdB} - (2 * (2 * (456\,149 * \text{JpA} - 1\,778\,067 * \text{JpB} + 1\,222\,938 * \text{JdC}) * \text{JdC} + \\
& 1\,837\,511 * \text{JpA}^2 - 1\,011\,458 * \text{JpA} * \text{JpB} + 1\,837\,511 * \text{JpB}^2) *
\end{aligned}$$

$$\begin{aligned}
& \text{JdC} + 48\,696 * \text{JpA}^3 - 1\,907\,161 * \text{JpA}^2 * \text{JpB} + \\
& 519\,309 * \text{JpA} * \text{JpB}^2 - 597\,289 * \text{JpB}^3) * \text{JdB} + \\
4 * & ((36 * (67\,043 * \text{JpA} - 7128 * \text{JpB} + 4644 * \text{JdC}) * \text{JdC} + \\
& 616\,315 * \text{JpA}^2 - 3\,520\,962 * \text{JpA} * \text{JpB} + 213\,624 * \text{JpB}^2) * \text{JdC} + \\
& 597\,289 * \text{JpA}^3 - 519\,309 * \text{JpA}^2 * \text{JpB} + 1\,907\,161 * \text{JpA} * \text{JpB}^2 - \\
& 48\,696 * \text{JpB}^3) * \text{JdC} - (123\,612 * \text{JpA}^4 + 1\,536\,150 * \text{JpA}^3 * \text{JpB} - \\
& 118\,955 * \text{JpA}^2 * \text{JpB}^2 + 1\,536\,150 * \text{JpA} * \text{JpB}^3 + 123\,612 * \text{JpB}^4) - \\
(2 * & (4 * (177\,724 * \text{JpA} + 3867 * \text{JpB} - 38\,622 * \text{JdC}) * \text{JdC}^2 + \\
& 49 * (3669 * \text{JpA}^2 - 4157 * \text{JpA} * \text{JpB} + 3669 * \text{JpB}^2) * (\text{JpA} + \text{JpB}) + \\
& 2 * (241\,928 * \text{JpA}^2 - 146\,692 * \text{JpA} * \text{JpB} - 138\,609 * \text{JpB}^2) * \text{JdC} + \\
& 2 * (2 * (3867 * \text{JpA} + 177\,724 * \text{JpB} + 76\,672 * \text{JdC} - 38\,622 * \text{JdB}) * \\
& \text{JdB} - (64 * (6733 * (\text{JpA} + \text{JpB}) - 2396 * \text{JdC}) * \text{JdC} + 138\,609 * \\
& \text{JpA}^2 + 146\,692 * \text{JpA} * \text{JpB} - 241\,928 * \text{JpB}^2)) * \text{JdB}) + \\
(2271 * & \text{Ja}^2 - 678\,128 * \text{JdB}^2 - 1\,095\,952 * \text{JdB} * \text{JdC} + \\
& 619\,952 * \text{JdB} * \text{JpA} - 37\,112 * \text{JdB} * \text{JpB} - 678\,128 * \text{JdC}^2 - \\
& 37\,112 * \text{JdC} * \text{JpA} + 619\,952 * \text{JdC} * \text{JpB} - 433\,836 * \text{JpA}^2 + \\
& 78\,436 * \text{JpA} * \text{JpB} - 433\,836 * \text{JpB}^2) * \text{Ja}) * \text{Ja}) * \text{Ja} + \\
2 * & (2 * (6 * (108 * (1888 * \text{JpA} - 619 * \text{JpB} + 362 * \text{JdC} - 1216 * \text{JdB}) * \\
& \text{JdB} - (108 * (5161 * \text{JdC} - 132 * \text{JpA} - 5733 * \text{JpB}) * \text{JdC} + \\
& 55\,872 * \text{JpA}^2 - 101\,640 * \text{JpA} * \text{JpB} + 162\,683 * \text{JpB}^2)) * \text{JdB} + \\
& 2 * (162 * (5157 * (\text{JpA} + \text{JpB}) - 10\,322 * \text{JdC}) * \text{JdC} - \\
& (248\,724 * \text{JpA}^2 + 899\,822 * \text{JpA} * \text{JpB} - 607\,829 * \text{JpB}^2)) * \\
& \text{JdC} - (334\,656 * \text{JpA}^3 + 258\,084 * \text{JpA}^2 * \text{JpB} - \\
& 498\,697 * \text{JpA} * \text{JpB}^2 + 488\,729 * \text{JpB}^3)) * \text{JdB} + \\
4 * & (324 * (362 * \text{JdC} + 5733 * \text{JpA} + 132 * \text{JpB}) * \text{JdC}^2 + \\
& (104\,628 * \text{JpA}^2 - 816\,569 * \text{JpA} * \text{JpB} + 104\,628 * \text{JpB}^2) * (\text{JpA} + \text{JpB}) + \\
& (607\,829 * \text{JpA}^2 - 899\,822 * \text{JpA} * \text{JpB} - 248\,724 * \text{JpB}^2) * \text{JdC}) * \text{JdC} + \\
& 367\,104 * \text{JpA}^4 + 100\,632 * \text{JpA}^3 * \text{JpB} + 687\,865 * \text{JpA}^2 * \text{JpB}^2 + \\
& 1160\,142 * \text{JpA} * \text{JpB}^3 + 22\,074 * \text{JpB}^4) * \text{JdB} - \\
(2 * & (2 * (6 * (108 * (619 * \text{JpA} - 1888 * \text{JpB} + 1216 * \text{JdC}) * \text{JdC} + \\
& 162\,683 * \text{JpA}^2 - 101\,640 * \text{JpA} * \text{JpB} + 55\,872 * \text{JpB}^2) * \\
& \text{JdC} + 488\,729 * \text{JpA}^3 - 498\,697 * \text{JpA}^2 * \text{JpB} + \\
& 258\,084 * \text{JpA} * \text{JpB}^2 + 334\,656 * \text{JpB}^3) * \text{JdC} - \\
& (22\,074 * \text{JpA}^4 + 1160\,142 * \text{JpA}^3 * \text{JpB} + 687\,865 * \text{JpA}^2 * \\
& \text{JpB}^2 + 100\,632 * \text{JpA} * \text{JpB}^3 + 367\,104 * \text{JpB}^4)) * \text{JdC} + \\
& (59\,648 * \text{JpA}^4 - 6474 * \text{JpA}^3 * \text{JpB} + 547\,083 * \text{JpA}^2 * \text{JpB}^2 - \\
& 6474 * \text{JpA} * \text{JpB}^3 + 59\,648 * \text{JpB}^4) * (\text{JpA} + \text{JpB})) + \\
2 * & ((4 * (4 * (106\,594 * \text{JpA} + 2997 * \text{JpB} - 9234 * \text{JdC}) * \text{JdC}^2 + (42\,647 * \\
& \text{JpA}^2 - 101\,251 * \text{JpA} * \text{JpB} + 42\,647 * \text{JpB}^2) * (\text{JpA} + \text{JpB}) + \\
& 2 * (123\,602 * \text{JpA}^2 - 57\,374 * \text{JpA} * \text{JpB} - 46\,123 * \text{JpB}^2) * \text{JdC} + \\
& 2 * (2 * (2997 * \text{JpA} + 106\,594 * \text{JpB} - 28\,836 * \text{JdC} - 9234 * \text{JdB}) * \\
& \text{JdB} - (8 * (21\,161 * (\text{JpA} + \text{JpB}) + 7209 * \text{JdC}) * \text{JdC} + 46\,123 * \\
& \text{JpA}^2 + 57\,374 * \text{JpA} * \text{JpB} - 123\,602 * \text{JpB}^2)) * \text{JdB}) - \\
& (258\,913 * \text{Ja}^2 + 876\,624 * \text{JdB}^2 + 2\,251\,728 * \text{JdB} * \text{JdC} - \\
& 1\,056\,912 * \text{JdB} * \text{JpA} - 279\,640 * \text{JdB} * \text{JpB} + 876\,624 * \text{JdC}^2 - \\
& 279\,640 * \text{JdC} * \text{JpA} - 1\,056\,912 * \text{JdC} * \text{JpB} + 908\,324 * \text{JpA}^2 +
\end{aligned}$$

$$\begin{aligned}
& 633\,164 * JpA * JpB + 908\,324 * JpB^2) * Ja) * Ja - \\
(4 * (3 * (108 * (2599 * JpA - 760 * JpB + 500 * JdC) * JdC + \\
& 136\,581 * JpA^2 - 408\,118 * JpA * JpB + 56\,904 * JpB^2) * JdC + \\
& 189\,303 * JpA^3 - 385\,051 * JpA^2 * JpB + 635\,605 * JpA * JpB^2 - \\
& 35\,544 * JpB^3) * JdC - (65\,580 * JpA^4 + 513\,958 * JpA^3 * JpB - \\
& 190\,763 * JpA^2 * JpB^2 + 513\,958 * JpA * JpB^3 + 65\,580 * JpB^4) - \\
4 * (324 * (760 * JpA - 2599 * JpB + 5046 * JdC - 500 * JdB) * JdB^2 + \\
& 2 * (817\,452 * JdC^2 + 773\,550 * JdC * JpA - 1\,232\,658 * JdC * JpB + \\
& 620\,565 * JpA^2 - 816\,290 * JpA * JpB + 620\,565 * JpB^2) * \\
& JdC + 35\,544 * JpA^3 - 635\,605 * JpA^2 * JpB + \\
& 385\,051 * JpA * JpB^2 - 189\,303 * JpB^3 - 3 * \\
& (108 * (7609 * JpA - 4775 * JpB + 4299 * JdC) * JdC + 56\,904 * JpA^2 - \\
& 408\,118 * JpA * JpB + 136\,581 * JpB^2) * JdB) * JdB) - \\
2 * (324 * (1862 * JpA - 47 * JpB + 54 * JdC) * JdC^2 - \\
& (20\,293 * JpA^2 + 148\,705 * JpA * JpB + 20\,293 * JpB^2) * (JpA + JpB) + \\
& 2 * (176\,118 * JpA^2 - 16\,180 * JpA * JpB - 7087 * JpB^2) * JdC - \\
& 2 * (162 * (47 * JpA - 1862 * JpB + 1692 * JdC - 54 * JdB) * JdB + \\
& 648 * (251 * (JpA + JpB) + 423 * JdC) * JdC + 7087 * JpA^2 + \\
& 16\,180 * JpA * JpB - 176\,118 * JpB^2) * JdB + \\
& (663\,681 * Ja^2 - 780\,840 * JdB^2 + 379\,080 * JdB * JdC + \\
& 990\,792 * JdB * JpA - 506\,964 * JdB * JpB - 780\,840 * JdC^2 - \\
& 506\,964 * JdC * JpA + 990\,792 * JdC * JpB - 700\,394 * JpA^2 - \\
& 267\,614 * JpA * JpB - 700\,394 * JpB^2) * Ja - \\
2 * (162 * (586 * J2 - 5541 * Ja) * J2 + 1\,173\,601 * Ja^2 - \\
& 230\,040 * JdB^2 + 747\,144 * JdB * JdC + 300\,024 * JdB * JpA - \\
& 420\,228 * JdB * JpB - 230\,040 * JdC^2 - 420\,228 * JdC * JpA + \\
& 300\,024 * JdC * JpB - 153\,030 * JpA^2 + 102\,626 * JpA * JpB - \\
& 153\,030 * JpB^2) * J2) * J2) * J2) * J2) * J2 - \\
(2 * ((4 * ((4 * (920\,539 * JpA + 208\,041 * JpB - 300\,319 * JdC) * JdC - \\
& (651\,480 * JpA^2 + 1\,515\,578 * JpA * JpB + 77\,239 * JpB^2) + \\
& 4 * (150\,360 * JpA + 174\,383 * JpB - \\
& 490\,402 * JdC - 13\,428 * JdB) * JdB) * JdB + \\
& 2 * (2 * (208\,041 * JpA + 920\,539 * JpB - 490\,402 * JdC) * JdC - \\
& (935\,935 * JpA^2 + 282\,738 * JpA * JpB + 935\,935 * JpB^2) * \\
& JdC + 199\,992 * JpA^3 + 809\,497 * JpA^2 * JpB - \\
& 7215 * JpA * JpB^2 + 232\,069 * JpB^3) * JdB + \\
& 4 * ((4 * (174\,383 * JpA + 150\,360 * JpB - 13\,428 * JdC) * JdC - \\
& (77\,239 * JpA^2 + 1\,515\,578 * JpA * JpB + 651\,480 * JpB^2) * JdC + \\
& 232\,069 * JpA^3 - 7215 * JpA^2 * JpB + 809\,497 * JpA * JpB^2 + \\
& 199\,992 * JpB^3) * JdC - (32\,532 * JpA^4 + 409\,078 * JpA^3 * JpB - \\
& 224\,537 * JpA^2 * JpB^2 + 409\,078 * JpA * JpB^3 + 32\,532 * JpB^4) - \\
& (2 * (2 * (304\,586 * JpA + 270\,681 * JpB - 307\,770 * JdC) * JdC + \\
& 29\,442 * JpA^2 - 360\,484 * JpA * JpB - 9199 * JpB^2) * JdC - \\
& (102\,373 * JpA^2 - 46\,579 * JpA * JpB + 102\,373 * JpB^2) * \\
& (JpA + JpB) + 2 * (2 * (270\,681 * JpA + 304\,586 * JpB - \\
& 735\,060 * JdC - 307\,770 * JdB) * JdB +
\end{aligned}$$

$$\begin{aligned}
& 8 * (112\,031 * (JpA + JpB) - 183\,765 * JdC) * JdC - \\
& (9199 * JpA^2 + 360\,484 * JpA * JpB - 29\,442 * JpB^2) * JdB - \\
& (81\,557 * Ja^2 + 1\,020\,072 * JdB^2 + 2\,036\,440 * JdB * JdC - \\
& 951\,240 * JdB * JpA - 1\,140\,732 * JdB * JpB + 1\,020\,072 * JdC^2 - \\
& 1\,140\,732 * JdC * JpA - 951\,240 * JdC * JpB + 274\,458 * JpA^2 + \\
& 547\,534 * JpA * JpB + 274\,458 * JpB^2) * Ja) * Ja) * Ja + \\
2 * (4 * ((4 * (544\,273 * JpA + 222\,972 * JpB - 129\,062 * JdC) * JdC + \\
& 54\,965 * JpA^2 - 1\,893\,638 * JpA * JpB - 532\,644 * JpB^2) * JdC + \\
& (146\,652 * JpA^2 + 7067 * JpA * JpB + 146\,652 * JpB^2) * \\
& (JpA + JpB)) * JdC + 527\,136 * JpA^4 - 227\,736 * JpA^3 * JpB - \\
& 390\,511 * JpA^2 * JpB^2 + 248\,630 * JpA * JpB^3 - 57\,798 * JpB^4 + \\
2 * (2 * (4 * (273\,200 * JpA + 7893 * JpB - 129\,062 * JdC - 120\,224 * JdB) * \\
& JdB + 4 * (222\,972 * JpA + 544\,273 * JpB - 536\,189 * JdC) * JdC - \\
& (568\,064 * JpA^2 + 104\,952 * JpA * JpB + 464\,949 * JpB^2)) * JdB + \\
2 * (2 * (825\,201 * (JpA + JpB) - 1\,072\,378 * JdC) * JdC - \\
& (532\,644 * JpA^2 + 1\,893\,638 * JpA * JpB - 54\,965 * JpB^2)) * \\
& JdC - (240\,768 * JpA^3 - 217\,452 * JpA^2 * JpB - \\
& 919\,957 * JpA * JpB^2 + 211\,801 * JpB^3)) * JdB) * JdB + \\
2 * (2 * (2 * (4 * (7893 * JpA + 273\,200 * JpB - 120\,224 * JdC) * JdC - \\
& (464\,949 * JpA^2 + 104\,952 * JpA * JpB + 568\,064 * JpB^2)) * \\
& JdC - (211\,801 * JpA^3 - 919\,957 * JpA^2 * JpB - \\
& 217\,452 * JpA * JpB^2 + 240\,768 * JpB^3)) * JdC - \\
& (57\,798 * JpA^4 - 248\,630 * JpA^3 * JpB + 390\,511 * JpA^2 * \\
& JpB^2 + 227\,736 * JpA * JpB^3 - 527\,136 * JpB^4)) * JdC - \\
& (131\,936 * JpA^4 - 238\,970 * JpA^3 * JpB + 144\,755 * JpA^2 * JpB^2 - \\
& 238\,970 * JpA * JpB^3 + 131\,936 * JpB^4) * (JpA + JpB)) * Ja + \\
4 * ((4 * (2 * (4 * (77\,099 * JpA - 73\,872 * JpB + 37\,908 * JdC) * JdC^2 - \\
& (120\,092 * JpA^2 + 27\,555 * JpA * JpB - 1008 * JpB^2) * JpB + 4 * \\
& (121\,226 * JpA^2 - 32\,100 * JpA * JpB + 21\,491 * JpB^2) * JdC) - \\
& (360\,288 * JdB * JdC - 200\,272 * JdB * JpB + 400\,788 * JdC^2 + \\
& 266\,000 * JdC * JpA - 136\,300 * JdC * JpB + \\
& 71\,256 * JpA * JpB - 52\,011 * JpB^2) * JdB) * JdB - \\
& (8 * ((2 * (100\,197 * JdC + 147\,744 * JpA - 154\,198 * JpB) * JdC + \\
& 92\,743 * JpA^2 - 564\,988 * JpA * JpB + 92\,743 * JpB^2) * JdC + \\
& 233\,748 * JpA^3 - 43\,799 * JpA^2 * JpB + 177\,972 * JpA * JpB^2 + \\
& 25\,853 * JpB^3) * JdC - (513\,360 * JpA^3 + 22\,938 * JpA^2 * JpB - \\
& 26\,088 * JpA * JpB^2 + 54\,571 * JpB^3) * JpB)) * JdB - \\
& (8 * ((2 * ((90\,072 * JdC - 34\,075 * JpA + 66\,500 * JpB) * JdC - \\
& 2 * (21\,491 * JpA^2 - 32\,100 * JpA * JpB + 121\,226 * JpB^2)) * \\
& JdC + 25\,853 * JpA^3 + 177\,972 * JpA^2 * JpB - \\
& 43\,799 * JpA * JpB^2 + 233\,748 * JpB^3) * JdC - \\
& (16\,785 * JpA^4 + 11\,590 * JpA^3 * JpB + 42\,037 * JpA^2 * \\
& JpB^2 + 11\,590 * JpA * JpB^3 + 16\,785 * JpB^4)) * JdC + \\
& (29\,468 * JpA^4 + 10\,686 * JpA^3 * JpB - 34\,408 * JpA^2 * JpB^2 + \\
& 37\,057 * JpA * JpB^3 - 20\,716 * JpB^4) * JpB)) * JdB +
\end{aligned}$$

$$\begin{aligned}
& (4 * (4 * ((200272 * JdC + 52011 * JpA - 71256 * JpB) * JdC + \\
& \quad 2 * (1008 * JpA^2 - 27555 * JpA * JpB - 120092 * JpB^2))) * JdC + \\
& \quad 54571 * JpA^3 - 26088 * JpA^2 * JpB + 22938 * JpA * JpB^2 + \\
& \quad 513360 * JpB^3) * JdC^2 + \\
& \quad (9608 * JpA^4 + 77619 * JpA^3 * JpB + 35288 * JpA^2 * JpB^2 + \\
& \quad 77619 * JpA * JpB^3 + 9608 * JpB^4) * JpB + \\
& \quad 4 * (20716 * JpA^4 - 37057 * JpA^3 * JpB + 34408 * JpA^2 * JpB^2 - \\
& \quad 10686 * JpA * JpB^3 - 29468 * JpB^4) * JdC) * JpA) * Ja - \\
& (2 * (2 * (2 * (2 * (2 * (162 * (2148 * JpA + 13 * JpB - 34 * JdC) * JdC - \\
& \quad (261304 * JpA + 11987 * JpB) * JpB) * JdC + \\
& \quad 288360 * JpA^3 - 30940 * JpA * JpB^2 + 9711 * JpB^3 - \\
& \quad 8 * (324 * (83 * JdC - 65 * JpB) * JdC + 96066 * JpA^2 - \\
& \quad 853 * JpB^2 - 324 * (14 * JdB + 141 * JpA) * JdB) * JdB) * \\
& \quad JdB + 8 * (162 * (866 * (JpA + JpB) - 17 * JdC) * JdC^2 + \\
& \quad (52052 * JpA^2 + 4935 * JpA * JpB + 19645 * JpB^2) * JpB - \\
& \quad (71932 * JpA^2 + 67958 * JpA * JpB + 119839 * JpB^2) * JdC) * \\
& \quad JdC + 288360 * JpA^4 + 23944 * JpA^2 * JpB^2 - \\
& \quad 54516 * JpA * JpB^3 + 2839 * JpB^4) * JdB + 4 * \\
& \quad (2 * (162 * (13 * JpA + 2148 * JpB - 664 * JdC) * JdC^2 - \\
& \quad (49500 * JpA^2 - 144011 * JpA * JpB + 49500 * JpB^2) * \\
& \quad (JpA + JpB) - 2 * (119839 * JpA^2 + 67958 * JpA * JpB + \\
& \quad 71932 * JpB^2) * JdC) * JdC + (4680 * JpA^3 - 43069 * JpA^2 * \\
& \quad JpB - 13510 * JpA * JpB^2 + 51042 * JpB^3) * JpB) * \\
& \quad JdC - (384264 * JpA^5 - 176776 * JpA^3 * JpB^2 - 177258 * \\
& \quad JpA^2 * JpB^3 + 10867 * JpA * JpB^4 + 14636 * JpB^5)) * JdB - \\
& (8 * (2 * (11987 * JpA + 261304 * JpB - 84240 * JdC) * JdC^3 - \\
& \quad (2090 * JpA^2 + 10321 * JpA * JpB + 2090 * JpB^2) * (JpA + JpB) * \\
& \quad JpB - 4 * (19645 * JpA^2 + 4935 * JpA * JpB + 52052 * JpB^2) * \\
& \quad JdC^2 - (51042 * JpA^3 - 13510 * JpA^2 * JpB - \\
& \quad 43069 * JpA * JpB^2 + 4680 * JpB^3) * JdC) * JdC - \\
& \quad (91368 * JpA^5 - 169756 * JpA^3 * JpB^2 - 80532 * JpA^2 * \\
& \quad JpB^3 + 54229 * JpA * JpB^4 + 9896 * JpB^5)) * JpA) * JdB + \\
& 2 * (4 * (2 * (8 * (324 * (14 * JdC + 141 * JpB) * JdC + 853 * JpA^2 - \\
& \quad 96066 * JpB^2) * JdC + 9711 * JpA^3 - 30940 * JpA^2 * JpB + \\
& \quad 288360 * JpB^3) * JdC + 2839 * JpA^4 - 54516 * JpA^3 * \\
& \quad JpB + 23944 * JpA^2 * JpB^2 + 288360 * JpB^4) * JdC^2 + \\
& \quad (9896 * JpA^5 + 54229 * JpA^4 * JpB - 80532 * JpA^3 * JpB^2 - \\
& \quad 169756 * JpA^2 * JpB^3 + 91368 * JpB^5) * JpB - \\
& \quad 2 * (14636 * JpA^5 + 10867 * JpA^4 * JpB - 177258 * JpA^3 * \\
& \quad JpB^2 - 176776 * JpA^2 * JpB^3 + 384264 * JpB^5) * JdC) * JdC + \\
& (4536 * JpA^6 - 4536 * JpA^5 * JpB - 7220 * JpA^4 * JpB^2 - \\
& \quad 67117 * JpA^3 * JpB^3 - \\
& \quad 7220 * JpA^2 * JpB^4 - 4536 * JpA * JpB^5 + \\
& \quad 4536 * JpB^6) * (JpA + JpB))) / 113246208;
\end{aligned}$$
